# Supplementary material for: Quantifier Elimination for Normal Cone Computations
Source: arXiv:2402.05579 ancillary file (2024-02-08)
Supplement: Supplementary file 1 [file QE_NormalCone_Calculations_PDF.pdf]

This notebook accompanies the paper:

**“Quantifier Elimination for Normal Cone Computations” by Michael Mandlmayr and Ali Kemal Uncu**

In this notebook, we present the explicit computations that exemplifies the main algorithms. The paper and the most current version of this notebook can be found on the Second authors website: [www.akuncu.com](http://www.akuncu.com).

This code is originally run on a computer with : Processor AMD A12 - 9720 P RADEON R7, 12 COMPUTE CORES 4 C + 8 G, 2700 Mhz, 4 Core (s), 4 Logical Processor (s), with 32.0 GB Installed Physical Memory (RAM) .

The times shown are from that run .

## Disjunctive Normal Form function:

```
(*
Takes logical formula with conjunctions( $\wedge$ ) and disjunctions( $\vee$ ) and gives a disjunction
of conjunctions (other vocabulary: "...gives or/union of and/intersection statements")
*)

In[1]:= DNFexp[e_Or] := DNFexp /@ e
DNFexp[And[a___, b_Or, c___]] := DNFexp[And[a, #, c]] & /@ b
DNFexp[other_] := other

(* Example: *)

In[4]:= DNFexp[(a < 0 && b ≤ 0 && c == 0) || (b == 0 && ((a ≤ 0 && c ≥ 0) || (a > 0 && c > 0)))]
Out[4]= (a < 0 && b ≤ 0 && c == 0) || (b == 0 && a ≤ 0 && c ≥ 0) || (b == 0 && a > 0 && c > 0)
```

# Calculating Normal Cones

Example 1 : 1 Dimensional Example :  $C = \{y: y \geq 0\}$

```
In[5]:= clause = ForAll[Eps, Eps > 0, Exists[del,
  del > 0,
  ForAll[x, x ≥ 0 && x ≠ X && Sqrt[(x - X)^2] < del, ((V(x - X) < Eps Sqrt[(x - X)^2] || V(x - X) ≤ 0)
  )]]]
```

```
Out[5]=  $\forall \text{Eps}, \text{Eps} > 0 \exists \text{del}, \text{del} > 0 \forall_{x, x \geq 0 \&\& x \neq X \&\& \sqrt{(x-X)^2} < \text{del}} \left( V(x - X) < \text{Eps} \sqrt{(x - X)^2} \parallel V(x - X) \leq 0 \right)$ 
```

```
In[6]:= Timing[CylindricalDecomposition[clause, {x, X, Eps, del, V}]]
```

```
Out[6]= {1.83924, X < 0 || (X == 0 && V ≤ 0) || (X > 0 && V == 0)}
```

## 2D Example : KKT conditions

Showing that we cannot do QE on the whole problem directly.

```
In[7]:= clause = ForAll[Eps, Eps > 0, Exists[del,
  del > 0,
  ForAll[{x, y}, x ≥ 0 && (y + x^2)(y - x^2) == 0 && x ≠ X && y ≠ Y && Sqrt[(x - X)^2 + (y - Y)^2] < del,
  ((v1(x - X) + v2(y - Y) < Eps Sqrt[(x - X)^2 + (y - Y)^2] || v1(x - X) + v2(y - Y) ≤ 0)
  )]]]
```

```
Out[7]=  $\forall \text{Eps}, \text{Eps} > 0 \exists \text{del}, \text{del} > 0 \forall_{\{x, y\}, x \geq 0 \&\& (-x^2 + y)(x^2 + y) = 0 \&\& x \neq X \&\& y \neq Y \&\& \sqrt{(x-X)^2 + (y-Y)^2} < \text{del}} \left( v1(x - X) + v2(y - Y) < \text{Eps} \sqrt{(x - X)^2 + (y - Y)^2} \parallel v1(x - X) + v2(y - Y) \leq 0 \right)$ 
```

```
In[8]:= Timing[Resolve[%, Reals]] (* Does not terminate in 24 hrs *)
```

```
Out[8]= $Aborted
```

## Example 2: Showing that (-1,-1) is in $N_C(0,0)$ :

```
In[9]:= clause = ForAll[Eps, Eps > 0, Exists[del,
    del > 0,
    ForAll[{x, y}, x ≥ 0 && (y + x^2)(y - x^2) == 0 && x ≠ X && y ≠ Y && Sqrt[(x - X)^2 + (y - Y)^2] < del,
        ((v1(x - X) + v2(y - Y)) < Eps Sqrt[(x - X)^2 + (y - Y)^2] || v1(x - X) + v2(y - Y) ≤ 0)
    ]]] /. {X → 0, Y → 0} /. {v1 → -1, v2 → -1}
```

```
Out[9]=  $\forall \text{Eps}, \text{Eps} > 0 \exists \text{del}, \text{del} > 0 \forall \{x, y\}, x \geq 0 \&\& (-x^2 + y)(x^2 + y) = 0 \&\& x \neq 0 \&\& y \neq 0 \&\& \sqrt{x^2 + y^2} < \text{del} \left( -x - y < \text{Eps} \sqrt{x^2 + y^2} \parallel -x - y \leq 0 \right)$ 
```

```
In[10]:= Timing[Reduce[clause, Reals]]
```

```
Out[10]= {0.774426, True}
```

## Example 4: Normal cone $N_C(0,0)$ calculated one cell at a time and combining later

(\* The clause to reduce \*)

```
In[11]:=  $\forall \text{Eps}, \text{Eps} > 0 \exists \text{del}, \text{del} > 0 \forall \{x, y\}, x \geq 0 \&\& (-x^2 + y)(x^2 + y) = 0 \&\& x \neq X \&\& y \neq Y \&\& \sqrt{(x - X)^2 + (y - Y)^2} < \text{del} \left( v1(x - X) + v2(y - Y) < \text{Eps} \sqrt{(x - X)^2 + (y - Y)^2} \parallel v1(x - X) + v2(y - Y) \leq 0 \right) /. \{X \rightarrow 0, Y \rightarrow 0\}$ 
```

```
Out[11]=  $\forall \text{Eps}, \text{Eps} > 0 \exists \text{del}, \text{del} > 0 \forall \{x, y\}, x \geq 0 \&\& (-x^2 + y)(x^2 + y) = 0 \&\& x \neq 0 \&\& y \neq 0 \&\& \sqrt{x^2 + y^2} < \text{del} \left( x v1 + y v2 < \text{Eps} \sqrt{x^2 + y^2} \parallel x v1 + y v2 \leq 0 \right)$ 
```

(\* CAD of the constraint set C \*)

```
In[12]:= gph = DNFexp[CylindricalDecomposition[x ≥ 0 && (y + x^2)(y - x^2) == 0, {x, y}]]
```

```
Out[12]= (x == 0 && y == 0) || (x > 0 && y == -x^2) || (x > 0 && y == x^2)
```

**C1:  $x == y == 0$**

```
In[13]:= gph[[1]]
```

```
Out[13]= x == 0 && y == 0
```

(\* Clause in this case is trivial:

Mathematica complains that we entered Forall[{0,0},...],  
as 0 is not a variable. We can remove these and similar occurrences by hand.  
\*)

In[14]:=  $\forall \text{Eps}, \text{Eps} > 0 \exists \text{del}, \text{del} > 0 \forall \{x, y\}, x \geq 0 \&\& (-x^2 + y) (x^2 + y) = 0 \&\& x \neq 0 \&\& y \neq 0 \&\& \sqrt{x^2 + y^2} < \text{del} \left( x v1 + y v2 < \text{Eps} \sqrt{x^2 + y^2} \parallel x v1 + y v2 \leq 0 \right) /. \{x \rightarrow 0, y \rightarrow 0\}$

⋯ ForAll: Evaluation of

$\{ \text{Eps} > 0, \exists \text{del}, \text{del} > 0 \forall \{0, 0\}, 0 \geq 0 \&\& (0^2 + 0) (0^2 + 0) = 0 \&\& 0 \neq 0 \&\& 0 \neq 0 \&\& \sqrt{0^2 + 0^2} < \text{del} (0 v1 + 0 v2 < \text{Eps} \sqrt{0^2 + 0^2} \parallel 0 v1 + 0 v2 \leq 0) \}$  generated message(s)  
{Exists::msgs}.

Out[14]=

$\forall \text{Eps}, \text{Eps} > 0 \exists \text{del}, \text{del} > 0 \forall \{0, 0\}, 0 \geq 0 \&\& (-0^2 + 0) (0^2 + 0) = 0 \&\& 0 \neq 0 \&\& 0 \neq 0 \&\& \sqrt{0^2 + 0^2} < \text{del} (0 v1 + 0 v2 < \text{Eps} \sqrt{0^2 + 0^2} \parallel 0 v1 + 0 v2 \leq 0)$

(\* This quantified formula after getting rid of redundancies is the argument in following line and reduces to True:\*)

In[19]:= Timing[Reduce[ $\forall \text{Eps}, \text{Eps} > 0 \exists \text{del}, \text{del} > 0 \text{Implies}[\text{False}, 0]$ , Reals]]

Out[19]=

{0.001958, True}

## C2: $y = x^2$

In[20]:= **gph[3]**

Out[20]=

$x > 0 \&\& y == x^2$

(\* Mathematica complains about the Forall[{x,x^2},...] appearance. \*)

In[21]:=  $\forall \text{Eps}, \text{Eps} > 0 \exists \text{del}, \text{del} > 0 \forall \{x, y\}, x \geq 0 \&\& (-x^2 + y) (x^2 + y) = 0 \&\& x \neq 0 \&\& y \neq 0 \&\& \sqrt{x^2 + y^2} < \text{del} \left( x v1 + y v2 < \text{Eps} \sqrt{x^2 + y^2} \parallel x v1 + y v2 \leq 0 \right) /. \{y \rightarrow x^2\}$

⋯ ForAll: Evaluation of

$\{ \text{Eps} > 0, \exists \text{del}, \text{del} > 0 \forall \{x, x^2\}, \<1 \> (x v1 + \text{Power}[\<2 \>] v2 < \text{Eps} \sqrt{\text{Plus}[\<2 \>]} \parallel x v1 + \text{Power}[\<2 \>] v2 \leq 0) \}$   
generated message(s) {Exists::msgs}.

Out[21]=

$\forall \text{Eps}, \text{Eps} > 0 \exists \text{del}, \text{del} > 0 \forall \{x, x^2\}, x \geq 0 \&\& (-x^2 + x^2) (x^2 + x^2) = 0 \&\& x \neq 0 \&\& x^2 \neq 0 \&\& \sqrt{x^2 + (x^2)^2} < \text{del} \left( x v1 + x^2 v2 < \text{Eps} \sqrt{x^2 + (x^2)^2} \parallel x v1 + x^2 v2 \leq 0 \right)$

(\* Here is x^2 removed by hand and the resolution of the clause \*)

In[22]:= **Timing**[Reduce[

$$\forall \text{Eps}, \text{Eps} > 0 \exists \text{del}, \text{del} > 0 \forall \{x, x \geq 0 \&\& (-x^2 + x^2) (x^2 + x^2) = 0 \&\& x \neq 0 \&\& x^2 \neq 0 \&\& \sqrt{x^2 + (x^2)^2} < \text{del} \left( x \text{ v1} + x^2 \text{ v2} < \text{Eps} \sqrt{x^2 + (x^2)^2} \parallel x \text{ v1} + x^2 \text{ v2} \leq 0 \right), \text{Reals}]$$

Out[22]=

{0.963748, v1 ≤ 0}

### C3: y = -x^2

In[23]:= **gph**[2]

Out[23]=

x > 0 && y == -x^2

In[24]:=  $\forall \text{Eps}, \text{Eps} > 0 \exists \text{del}, \text{del} > 0 \forall \{x, y, x \geq 0 \&\& (-x^2 + y) (x^2 + y) = 0 \&\& x \neq 0 \&\& y \neq 0 \&\& \sqrt{x^2 + y^2} < \text{del} \left( x \text{ v1} + y \text{ v2} < \text{Eps} \sqrt{x^2 + y^2} \parallel x \text{ v1} + y \text{ v2} \leq 0 \right) /. \{y \rightarrow -x^2\}$

⋯ **ForAll**: Evaluation of

$$\left\{ \text{Eps} > 0, \exists \text{del}, \text{del} > 0 \forall \{x, -x^2, x \geq 0 \&\& (\text{Times}[\llbracket 2 \rrbracket] + \text{Times}[\llbracket 2 \rrbracket]) (\llbracket 1 \rrbracket) = 0 \&\& x \neq 0 \&\& -x^2 \neq 0 \&\& \sqrt{\text{Power}[\llbracket 2 \rrbracket] + \text{Power}[\llbracket 2 \rrbracket]} < \text{del} \left( x \text{ v1} + \llbracket 2 \rrbracket \gg \text{v2} < \text{Eps} \sqrt{\text{Plus}[\llbracket 2 \rrbracket]} \parallel x \text{ v1} + \llbracket 2 \rrbracket \gg \text{v2} \leq 0 \right) \right\} \text{ generated}$$

message(s) {Exists::msgs}.

Out[24]=

$$\forall \text{Eps}, \text{Eps} > 0 \exists \text{del}, \text{del} > 0 \forall \{x, -x^2, x \geq 0 \&\& (-x^2 - x^2) (x^2 - x^2) = 0 \&\& x \neq 0 \&\& -x^2 \neq 0 \&\& \sqrt{x^2 + (-x^2)^2} < \text{del} \left( x \text{ v1} - x^2 \text{ v2} < \text{Eps} \sqrt{x^2 + (-x^2)^2} \parallel x \text{ v1} - x^2 \text{ v2} \leq 0 \right)$$

In[25]:= **Timing**[

$$\text{Resolve}[\forall \text{Eps}, \text{Eps} > 0 \exists \text{del}, \text{del} > 0 \forall \{x, x \geq 0 \&\& (-x^2 - x^2) (x^2 - x^2) = 0 \&\& x \neq 0 \&\& -x^2 \neq 0 \&\& \sqrt{x^2 + (-x^2)^2} < \text{del} \left( x \text{ v1} - x^2 \text{ v2} < \text{Eps} \sqrt{x^2 + (-x^2)^2} \parallel x \text{ v1} - x^2 \text{ v2} \leq 0 \right), \text{Reals}]$$

Out[25]=

{0.839343, v1 ≤ 0}

### Combining the outcomes:

In[26]:= **Reduce**[True && v1 ≤ 0 && v1 ≤ 0]

Out[26]=

v1 ≤ 0

## Example 3: 2D Example

Centered at (X,Y) with X Y == 0 and X >= 0 and Y >= 0:

## Direct Attempt (Does Not Terminate)

```
In[27]:= X Y == 0 && X ≥ 0 && Y ≥ 0 && ForAll[Eps, Eps > 0, Exists[del,
del > 0, ForAll[{x, y}, x y == 0 && x ≥ 0 && y ≥ 0 && Sqrt[(x - X)^2 + (y - Y)^2] < del,
(v1 (x - X) + v2 (y - Y) < Eps Sqrt[(x - X)^2 + (y - Y)^2] || v1 (x - X) + v2 (y - Y) ≤ 0)
]]]
```

Out[27]=

X Y == 0 && X ≥ 0 && Y ≥ 0 &&

$\forall_{Eps, Eps > 0} \exists_{del, del > 0} \forall_{\{x, y\}, x y = 0 \&\& x \geq 0 \&\& y \geq 0 \&\& \sqrt{(x-X)^2 + (y-Y)^2} < del} (v1 (x - X) + v2 (y - Y) < Eps \sqrt{(x - X)^2 + (y - Y)^2} \parallel v1 (x - X) + v2 (y - Y) \leq 0)$

```
In[28]:= Timing[Resolve[%, Reals]] (* Does not terminate in 24 hrs *)
```

Out[28]=

\$Aborted

## Case 1: X==0

```
In[29]:= X Y == 0 && X ≥ 0 && Y ≥ 0 && ForAll[Eps, Eps > 0, Exists[del,
del > 0, ForAll[{x, y}, x y == 0 && x ≥ 0 && y ≥ 0 && Sqrt[(x - X)^2 + (y - Y)^2] < del,
(v1 (x - X) + v2 (y - Y) < Eps Sqrt[(x - X)^2 + (y - Y)^2] || v1 (x - X) + v2 (y - Y) ≤ 0)
]]] /. X → 0
```

Out[29]=

$Y \geq 0 \&\& \forall_{Eps, Eps > 0} \exists_{del, del > 0} \forall_{\{x, y\}, x y = 0 \&\& x \geq 0 \&\& y \geq 0 \&\& \sqrt{x^2 + (y-Y)^2} < del} (x v1 + v2 (y - Y) < Eps \sqrt{x^2 + (y - Y)^2} \parallel x v1 + v2 (y - Y) \leq 0)$

```
In[30]:= Timing[Reduce[%, Reals]]
```

Out[30]=

{2.84054, (v2 < 0 && v1 ≤ 0 && Y == 0) || (v2 == 0 && ((v1 ≤ 0 && Y ≥ 0) || (v1 > 0 && Y > 0))}

```
In[31]:= CylindricalDecomposition[%%[2] && X == 0, {X, Y, v1, v2}] // DNFexp
```

Out[31]=

(X == 0 && Y == 0 && v1 ≤ 0 && v2 ≤ 0) || (X == 0 && Y > 0 && v2 == 0)

## Case 2: $Y=0$

```
In[32]:= X Y == 0 && X ≥ 0 && Y ≥ 0 && ForAll[Eps, Eps > 0, Exists[del,
      del > 0, ForAll[{y, x}, x y == 0 && x ≥ 0 && y ≥ 0 && Sqrt[(x - X)^2 + (y - Y)^2] < del,
      (v1 (x - X) + v2 (y - Y) < Eps Sqrt[(x - X)^2 + (y - Y)^2] || v1 (x - X) + v2 (y - Y) ≤ 0)
      ]]] /. Y → 0
```

Out[32]=

$$X \geq 0 \ \&\& \ \forall_{Eps, Eps > 0} \ \exists_{del, del > 0} \ \forall_{\{y, x\}, y x = 0 \ \&\& \ x \geq 0 \ \&\& \ y \geq 0 \ \&\& \ \sqrt{y^2 + (x - X)^2} < del \ \left( y v_2 + v_1 (x - X) < Eps \sqrt{y^2 + (x - X)^2} \ \&\& \ y v_2 + v_1 (x - X) \leq 0 \right)$$

```
In[33]:= Timing[Resolve[%, Reals]]
```

Out[33]=

```
{2.15063, (v2 ≤ 0 && ((v1 < 0 && X == 0) || (v1 == 0 && X ≥ 0))) || (v2 > 0 && v1 == 0 && X > 0)}
```

```
In[34]:= CylindricalDecomposition[%[[2]] && Y == 0, {X, Y, v1, v2}] // DNFexp
```

Out[34]=

```
(X == 0 && Y == 0 && v1 ≤ 0 && v2 ≤ 0) || (X > 0 && Y == 0 && v1 == 0)
```

## Combining the two cases

```
In[35]:= Simplify[%31 || %34]
```

Out[35]=

```
(Y == 0 && ((v1 == 0 && X > 0) || (X == 0 && v1 ≤ 0 && v2 ≤ 0))) || (v2 == 0 && X == 0 && Y > 0)
```

# Example 5 : 6 Dimensional Coulomb Friction Normal Cone Calculations

## CAD calculations for the C defined in (5.3)

$C := \text{gph}(Q)$

```
In[36]:= Gph[x1_, x2_, x3_, x4_, x5_, x6_] :=
  x4 ≤ 0 &&
  x3 ≥ 0 &&
  (
    (x1^2 + x2^2 == 0 && x5^2 + x6^2 ≤ x4^2) ||
    (x1^2 + x2^2 ≠ 0 && x5 == -x4 x1 / Sqrt[(x1^2 + x2^2)] && x6 == -x4 x2 / Sqrt[(x1^2 + x2^2)])
  ) &&
  (
    (x3 == 0 && x4 ≤ 0) || (x3 > 0 && x4 == 0)
  );
```

```
In[37]:= Gph[x1, x2, x3, x4, x5, x6]
```

```
Out[37]=
```

$$x4 \leq 0 \ \&\& \ x3 \geq 0 \ \&\& \ \left( (x1^2 + x2^2 == 0 \ \&\& \ x5^2 + x6^2 \leq x4^2) \ || \ \left( x1^2 + x2^2 \neq 0 \ \&\& \ x5 == -\frac{x1 x4}{\sqrt{x1^2 + x2^2}} \ \&\& \ x6 == -\frac{x2 x4}{\sqrt{x1^2 + x2^2}} \right) \right) \ \&\& \ ((x3 == 0 \ \&\& \ x4 \leq 0) \ || \ (x3 > 0 \ \&\& \ x4 == 0))$$

```
In[38]:= (* Calculate a CAD for gph(Q) to get semialgebraic components *)
```

```
Timing[
```

```
  GphCAD = CylindricalDecomposition[Gph[x1, x2, x3, x4, x5, x6], {x1, x2, x3, x4, x5, x6}];]
```

```
Out[38]=
```

```
{0.362259, Null}
```



In[40]:= DNFexp[GphCAD] (\* DNF of gphCAD to see the cells better \*)

Out[40]=

$$\left( x_1 < 0 \ \&\& \ x_2 \leq 0 \ \&\& \ x_3 == 0 \ \&\& \ x_4 \leq 0 \ \&\& \ x_5 == -\sqrt{\frac{x_1^2 x_4^2}{x_1^2 + x_2^2}} \ \&\& \ x_6 == -\sqrt{x_4^2 - x_5^2} \right) \parallel$$

$$(x_1 < 0 \ \&\& \ x_2 \leq 0 \ \&\& \ x_3 > 0 \ \&\& \ x_4 == 0 \ \&\& \ x_5 == 0 \ \&\& \ x_6 == 0) \parallel$$

$$\left( x_1 < 0 \ \&\& \ x_2 > 0 \ \&\& \ x_3 == 0 \ \&\& \ x_4 < 0 \ \&\& \ x_5 == -\sqrt{\frac{x_1^2 x_4^2}{x_1^2 + x_2^2}} \ \&\& \ x_6 == \sqrt{x_4^2 - x_5^2} \right) \parallel$$

$$(x_1 < 0 \ \&\& \ x_2 > 0 \ \&\& \ x_3 == 0 \ \&\& \ x_4 == 0 \ \&\& \ x_5 == 0 \ \&\& \ x_6 == 0) \parallel$$

$$(x_1 < 0 \ \&\& \ x_2 > 0 \ \&\& \ x_3 > 0 \ \&\& \ x_4 == 0 \ \&\& \ x_5 == 0 \ \&\& \ x_6 == 0) \parallel$$

$$\left( x_1 == 0 \ \&\& \ x_2 < 0 \ \&\& \ x_3 == 0 \ \&\& \ x_4 \leq 0 \ \&\& \ x_5 == 0 \ \&\& \ x_6 == -\sqrt{x_4^2} \right) \parallel$$

$$(x_1 == 0 \ \&\& \ x_2 < 0 \ \&\& \ x_3 > 0 \ \&\& \ x_4 == 0 \ \&\& \ x_5 == 0 \ \&\& \ x_6 == 0) \parallel$$

$$\left( x_1 == 0 \ \&\& \ x_2 == 0 \ \&\& \ x_3 == 0 \ \&\& \ x_4 < 0 \ \&\& \ x_5 == x_4 \ \&\& \ x_6 == -\sqrt{x_4^2 - x_5^2} \right) \parallel$$

$$\left( x_1 == 0 \ \&\& \ x_2 == 0 \ \&\& \ x_3 == 0 \ \&\& \ x_4 < 0 \ \&\& \ x_4 < x_5 < -x_4 \ \&\& \ -\sqrt{x_4^2 - x_5^2} \leq x_6 \leq \sqrt{x_4^2 - x_5^2} \right) \parallel$$

$$\left( x_1 == 0 \ \&\& \ x_2 == 0 \ \&\& \ x_3 == 0 \ \&\& \ x_4 < 0 \ \&\& \ x_5 == -x_4 \ \&\& \ x_6 == -\sqrt{x_4^2 - x_5^2} \right) \parallel$$

$$(x_1 == 0 \ \&\& \ x_2 == 0 \ \&\& \ x_3 == 0 \ \&\& \ x_4 == 0 \ \&\& \ x_5 == 0 \ \&\& \ x_6 == 0) \parallel$$

$$(x_1 == 0 \ \&\& \ x_2 == 0 \ \&\& \ x_3 > 0 \ \&\& \ x_4 == 0 \ \&\& \ x_5 == 0 \ \&\& \ x_6 == 0) \parallel$$

$$\left( x_1 == 0 \ \&\& \ x_2 > 0 \ \&\& \ x_3 == 0 \ \&\& \ x_4 < 0 \ \&\& \ x_5 == 0 \ \&\& \ x_6 == \sqrt{x_4^2} \right) \parallel$$

$$(x_1 == 0 \ \&\& \ x_2 > 0 \ \&\& \ x_3 == 0 \ \&\& \ x_4 == 0 \ \&\& \ x_5 == 0 \ \&\& \ x_6 == 0) \parallel$$

$$(x_1 == 0 \ \&\& \ x_2 > 0 \ \&\& \ x_3 > 0 \ \&\& \ x_4 == 0 \ \&\& \ x_5 == 0 \ \&\& \ x_6 == 0) \parallel$$

$$\left( x_1 > 0 \ \&\& \ x_2 < 0 \ \&\& \ x_3 == 0 \ \&\& \ x_4 \leq 0 \ \&\& \ x_5 == \sqrt{\frac{x_1^2 x_4^2}{x_1^2 + x_2^2}} \ \&\& \ x_6 == -\sqrt{x_4^2 - x_5^2} \right) \parallel$$

$$(x_1 > 0 \ \&\& \ x_2 < 0 \ \&\& \ x_3 > 0 \ \&\& \ x_4 == 0 \ \&\& \ x_5 == 0 \ \&\& \ x_6 == 0) \parallel$$

$$\left( x_1 > 0 \ \&\& \ x_2 == 0 \ \&\& \ x_3 == 0 \ \&\& \ x_4 \leq 0 \ \&\& \ x_5 == -x_4 \ \&\& \ x_6 == -\sqrt{x_4^2 - x_5^2} \right) \parallel$$

$$(x_1 > 0 \ \&\& \ x_2 == 0 \ \&\& \ x_3 > 0 \ \&\& \ x_4 == 0 \ \&\& \ x_5 == 0 \ \&\& \ x_6 == 0) \parallel$$

$$\left( x_1 > 0 \ \&\& \ x_2 > 0 \ \&\& \ x_3 == 0 \ \&\& \ x_4 < 0 \ \&\& \ x_5 == \sqrt{\frac{x_1^2 x_4^2}{x_1^2 + x_2^2}} \ \&\& \ x_6 == \sqrt{x_4^2 - x_5^2} \right) \parallel$$

$$(x_1 > 0 \ \&\& \ x_2 > 0 \ \&\& \ x_3 == 0 \ \&\& \ x_4 == 0 \ \&\& \ x_5 == 0 \ \&\& \ x_6 == 0) \parallel$$

$$(x_1 > 0 \ \&\& \ x_2 > 0 \ \&\& \ x_3 > 0 \ \&\& \ x_4 == 0 \ \&\& \ x_5 == 0 \ \&\& \ x_6 == 0) \parallel$$

In[41]:= Length[%] (\* DNF has 22 components \*)

Out[41]=

22

## CAD of $\text{gph}(Q)$ in DNF form

In[42]:= **GphCADSim = DNFExp[GphCAD]**(\* We would rather work with the DNF form of GphCAD \*)

Out[42]=

$$\left( x_1 < 0 \ \&\& \ x_2 \leq 0 \ \&\& \ x_3 == 0 \ \&\& \ x_4 \leq 0 \ \&\& \ x_5 == -\sqrt{\frac{x_1^2 x_4^2}{x_1^2 + x_2^2}} \ \&\& \ x_6 == -\sqrt{x_4^2 - x_5^2} \right) \parallel$$

$$(x_1 < 0 \ \&\& \ x_2 \leq 0 \ \&\& \ x_3 > 0 \ \&\& \ x_4 == 0 \ \&\& \ x_5 == 0 \ \&\& \ x_6 == 0) \parallel$$

$$\left( x_1 < 0 \ \&\& \ x_2 > 0 \ \&\& \ x_3 == 0 \ \&\& \ x_4 < 0 \ \&\& \ x_5 == -\sqrt{\frac{x_1^2 x_4^2}{x_1^2 + x_2^2}} \ \&\& \ x_6 == \sqrt{x_4^2 - x_5^2} \right) \parallel$$

$$(x_1 < 0 \ \&\& \ x_2 > 0 \ \&\& \ x_3 == 0 \ \&\& \ x_4 == 0 \ \&\& \ x_5 == 0 \ \&\& \ x_6 == 0) \parallel$$

$$(x_1 < 0 \ \&\& \ x_2 > 0 \ \&\& \ x_3 > 0 \ \&\& \ x_4 == 0 \ \&\& \ x_5 == 0 \ \&\& \ x_6 == 0) \parallel$$

$$\left( x_1 == 0 \ \&\& \ x_2 < 0 \ \&\& \ x_3 == 0 \ \&\& \ x_4 \leq 0 \ \&\& \ x_5 == 0 \ \&\& \ x_6 == -\sqrt{x_4^2} \right) \parallel$$

$$(x_1 == 0 \ \&\& \ x_2 < 0 \ \&\& \ x_3 > 0 \ \&\& \ x_4 == 0 \ \&\& \ x_5 == 0 \ \&\& \ x_6 == 0) \parallel$$

$$\left( x_1 == 0 \ \&\& \ x_2 == 0 \ \&\& \ x_3 == 0 \ \&\& \ x_4 < 0 \ \&\& \ x_5 == x_4 \ \&\& \ x_6 == -\sqrt{x_4^2 - x_5^2} \right) \parallel$$

$$\left( x_1 == 0 \ \&\& \ x_2 == 0 \ \&\& \ x_3 == 0 \ \&\& \ x_4 < 0 \ \&\& \ x_4 < x_5 < -x_4 \ \&\& \ -\sqrt{x_4^2 - x_5^2} \leq x_6 \leq \sqrt{x_4^2 - x_5^2} \right) \parallel$$

$$\left( x_1 == 0 \ \&\& \ x_2 == 0 \ \&\& \ x_3 == 0 \ \&\& \ x_4 < 0 \ \&\& \ x_5 == -x_4 \ \&\& \ x_6 == -\sqrt{x_4^2 - x_5^2} \right) \parallel$$

$$(x_1 == 0 \ \&\& \ x_2 == 0 \ \&\& \ x_3 == 0 \ \&\& \ x_4 == 0 \ \&\& \ x_5 == 0 \ \&\& \ x_6 == 0) \parallel$$

$$(x_1 == 0 \ \&\& \ x_2 == 0 \ \&\& \ x_3 > 0 \ \&\& \ x_4 == 0 \ \&\& \ x_5 == 0 \ \&\& \ x_6 == 0) \parallel$$

$$\left( x_1 == 0 \ \&\& \ x_2 > 0 \ \&\& \ x_3 == 0 \ \&\& \ x_4 < 0 \ \&\& \ x_5 == 0 \ \&\& \ x_6 == \sqrt{x_4^2} \right) \parallel$$

$$(x_1 == 0 \ \&\& \ x_2 > 0 \ \&\& \ x_3 == 0 \ \&\& \ x_4 == 0 \ \&\& \ x_5 == 0 \ \&\& \ x_6 == 0) \parallel$$

$$(x_1 == 0 \ \&\& \ x_2 > 0 \ \&\& \ x_3 > 0 \ \&\& \ x_4 == 0 \ \&\& \ x_5 == 0 \ \&\& \ x_6 == 0) \parallel$$

$$\left( x_1 > 0 \ \&\& \ x_2 < 0 \ \&\& \ x_3 == 0 \ \&\& \ x_4 \leq 0 \ \&\& \ x_5 == \sqrt{\frac{x_1^2 x_4^2}{x_1^2 + x_2^2}} \ \&\& \ x_6 == -\sqrt{x_4^2 - x_5^2} \right) \parallel$$

$$(x_1 > 0 \ \&\& \ x_2 < 0 \ \&\& \ x_3 > 0 \ \&\& \ x_4 == 0 \ \&\& \ x_5 == 0 \ \&\& \ x_6 == 0) \parallel$$

$$\left( x_1 > 0 \ \&\& \ x_2 == 0 \ \&\& \ x_3 == 0 \ \&\& \ x_4 \leq 0 \ \&\& \ x_5 == -x_4 \ \&\& \ x_6 == -\sqrt{x_4^2 - x_5^2} \right) \parallel$$

$$(x_1 > 0 \ \&\& \ x_2 == 0 \ \&\& \ x_3 > 0 \ \&\& \ x_4 == 0 \ \&\& \ x_5 == 0 \ \&\& \ x_6 == 0) \parallel$$

$$\left( x_1 > 0 \ \&\& \ x_2 > 0 \ \&\& \ x_3 == 0 \ \&\& \ x_4 < 0 \ \&\& \ x_5 == \sqrt{\frac{x_1^2 x_4^2}{x_1^2 + x_2^2}} \ \&\& \ x_6 == \sqrt{x_4^2 - x_5^2} \right) \parallel$$

$$(x_1 > 0 \ \&\& \ x_2 > 0 \ \&\& \ x_3 == 0 \ \&\& \ x_4 == 0 \ \&\& \ x_5 == 0 \ \&\& \ x_6 == 0) \parallel$$

$$(x_1 > 0 \ \&\& \ x_2 > 0 \ \&\& \ x_3 > 0 \ \&\& \ x_4 == 0 \ \&\& \ x_5 == 0 \ \&\& \ x_6 == 0) \parallel$$

## Normal cone calculations

### Set-up functions:

```
(* clause[CAD_cell] function takes a CAD cell and
writes the quantified formula (4.2) of Definition 7.*)
ClearAll[clause]
clause[GP_] :=
  ForAll[Eps, Eps > 0, Exists[del,
    del > 0, ForAll[{x1, x2, x3, x4, x5, x6}, GP && Sqrt[x52 + x62 + x42 + x12 + x22 + x32] < del,
      ((v1 x1 + v2 x2 + v3 x3 + V x4 + g1 x5 + g2 x6) < Eps Sqrt[x52 + x62 + x42 + x12 + x22 + x32] ||
        v1 x1 + v2 x2 + v3 x3 + V x4 + g1 x5 + g2 x6 ≤ 0)
    ]]]
```

In[45]:= **GphCADSim[5]**

Out[45]=

$x1 < 0 \ \&\& \ x2 > 0 \ \&\& \ x3 > 0 \ \&\& \ x4 == 0 \ \&\& \ x5 == 0 \ \&\& \ x6 == 0$

In[46]:= **clause[GphCADSim[5]]**

Out[46]=

$$\forall \text{Eps}, \text{Eps} > 0 \ \exists \text{del}, \text{del} > 0 \ \forall_{\{x1, x2, x3, x4, x5, x6\}, x1 < 0 \ \&\& \ x2 > 0 \ \&\& \ x3 > 0 \ \&\& \ x4 == 0 \ \&\& \ x5 == 0 \ \&\& \ x6 == 0 \ \&\& \ \sqrt{x1^2 + x2^2 + x3^2 + x4^2 + x5^2 + x6^2} < \text{del}} \left( \text{g1} \right. \\ \left. x5 + \text{g2} x6 + x4 V + x1 v1 + x2 v2 + x3 v3 < \right. \\ \left. \text{Eps} \sqrt{x1^2 + x2^2 + x3^2 + x4^2 + x5^2 + x6^2} \ \parallel \ \text{g1} x5 + \text{g2} x6 + x4 V + x1 v1 + x2 v2 + x3 v3 \leq 0 \right)$$

```

In[47]:= (* splt[CAD_cell] function takes in a cad_cell of DNF of gph(Q)
and puts it in the Normal cone definition while it makes obvious
equational constraint substitutions to simplify the logical clause *)
Clear[splt]
splt[cl_] := Module[
  {split, eqs, ineqs, i, vars},
  eqs = {};
  ineqs = {};
  Do[
    If[Head[cl[[i]]] === Equal && Head[cl[[i, 1]]] === Symbol,
      AppendTo[eqs, cl[[i][1] -> cl[[i][2]]], AppendTo[ineqs, cl[[i]]]
    (*Print[{cl[[i]], Head[cl[[i]], Head[cl[[i]]], ineqs}];*)
    ,
    {i, 6}];
  split = {Reduce`FreeVariables[ineqs], And @@ ineqs, eqs};
  (*Print[split]; Print[split[[1]]; *)
  Return[ForAll[Eps, Eps > 0, Exists[del,
    del > 0, ForAll1[split[[1]], split[[2]] && Sqrt[x52 + x62 + x42 + x12 + x22 + x32] < del,
    ((v1 x1 + v2 x2 + v3 x3 + V x4 + g1 x5 + g2 x6) < Eps Sqrt[x52 + x62 + x42 + x12 + x22 + x32] ||
    v1 x1 + v2 x2 + v3 x3 + V x4 + g1 x5 + g2 x6 ≤ 0)
    ]]] // . split[[3]] /. ForAll1 -> ForAll]
  ]

```

In[49]:= GphCADSim[5]

Out[49]=

$$x1 < 0 \ \&\& \ x2 > 0 \ \&\& \ x3 > 0 \ \&\& \ x4 == 0 \ \&\& \ x5 == 0 \ \&\& \ x6 == 0$$

In[50]:= splt[GphCADSim[5]]

Out[50]=

$$\forall_{Eps, Eps > 0} \exists_{del, del > 0} \forall_{\{x1, x2, x3\}, x1 < 0 \ \&\& \ x2 > 0 \ \&\& \ x3 > 0 \ \&\& \ \sqrt{x1^2 + x2^2 + x3^2} < del} \left( x1 v1 + x2 v2 + x3 v3 < \right. \\ \left. Eps \sqrt{x1^2 + x2^2 + x3^2} \ \parallel \ x1 v1 + x2 v2 + x3 v3 \leq 0 \right)$$

In[51]:= (\* Compare this with clause[GphCADSim[5]]:\*)

clause[GphCADSim[5]]

Out[51]=

$$\forall_{Eps, Eps > 0} \exists_{del, del > 0} \forall_{\{x1, x2, x3, x4, x5, x6\}, x1 < 0 \ \&\& \ x2 > 0 \ \&\& \ x3 > 0 \ \&\& \ x4 == 0 \ \&\& \ x5 == 0 \ \&\& \ x6 == 0 \ \&\& \ \sqrt{x1^2 + x2^2 + x3^2 + x4^2 + x5^2 + x6^2} < del} \left( g1 \right. \\ \left. x5 + g2 x6 + x4 V + x1 v1 + x2 v2 + x3 v3 < \right. \\ \left. Eps \sqrt{x1^2 + x2^2 + x3^2 + x4^2 + x5^2 + x6^2} \ \parallel \ g1 x5 + g2 x6 + x4 V + x1 v1 + x2 v2 + x3 v3 \leq 0 \right)$$

(\* x4==0&&x5==0&&x6==0

in the innermost quantified formula is

substituted in the simplification splt[CAD\_cell] function. \*)

## Running QuantifierElimination (QE) with a T second timer on the cells of DNF CAD

```
In[52]:= T = 1; (* Time limit is set to a single second *)
res = {}; (* Conditions found for v*'2*)
ind = {}; (* The indices of CAD cells which we
couldn't finish the QE calculations within the time frame *)
Do[
  tres = $Aborted;
  Print[Style[{i, GphCADSim[[i]], Red}];
  (* Prints the index and the description of the combined cell in Red*)
  Print[Style[Simplify[splt[GphCADSim[[i]]], Blue]];
  (* Prints the Normal cone definition structure QE needs to colx4e*)
  Print[TimeConstrained[Timing[tres = Resolve[splt[GphCADSim[[i]]], Reals]], T]];
  (*Tries QE and prints the outcome *)
  If[tres != $Aborted, AppendTo[res, tres], AppendTo[ind, i]];
  (*If the calculation yielded a solution,
records this in res, add indices of failed cells to ind*)
  ,
  {i, 1, 22}]
(* res is the pool of conditions that overestimates the normal cone for gph(Q). *)
```

$$\{1, x_1 < 0 \ \&\& \ x_2 \leq 0 \ \&\& \ x_3 == 0 \ \&\& \ x_4 \leq 0 \ \&\& \ x_5 == -\sqrt{\frac{x_1^2 x_4^2}{x_1^2 + x_2^2}} \ \&\& \ x_6 == -\sqrt{x_4^2 - x_5^2}\}$$

$$\forall_{\text{Eps}, \text{Eps} > 0} \exists_{\text{del}, \text{del} > 0} \forall_{(x_1, x_2, x_4), x_1 < 0 \ \&\& \ x_2 \leq 0 \ \&\& \ x_4 \leq 0 \ \&\& \ \sqrt{x_1^2 + x_2^2 + 2 x_4^2} < \text{del}} \left( -g_1 \sqrt{\frac{x_1^2 x_4^2}{x_1^2 + x_2^2}} - \right. \\ \left. g_2 \sqrt{x_4^2 - \frac{x_1^2 x_4^2}{x_1^2 + x_2^2}} + x_4 v_1 + x_1 v_1 + x_2 v_2 < \text{Eps} \sqrt{x_1^2 + x_2^2 + 2 x_4^2} \ \parallel \right. \\ \left. -g_1 \sqrt{\frac{x_1^2 x_4^2}{x_1^2 + x_2^2}} - g_2 \sqrt{x_4^2 - \frac{x_1^2 x_4^2}{x_1^2 + x_2^2}} + x_4 v_1 + x_1 v_1 + x_2 v_2 \leq 0 \right)$$

\$Aborted

$$\{2, x_1 < 0 \ \&\& \ x_2 \leq 0 \ \&\& \ x_3 > 0 \ \&\& \ x_4 == 0 \ \&\& \ x_5 == 0 \ \&\& \ x_6 == 0\}$$

$$\forall_{\text{Eps}, \text{Eps} > 0} \exists_{\text{del}, \text{del} > 0} \forall_{(x_1, x_2, x_3), x_1 < 0 \ \&\& \ x_2 \leq 0 \ \&\& \ x_3 > 0 \ \&\& \ \sqrt{x_1^2 + x_2^2 + x_3^2} < \text{del}} \left( x_1 v_1 + x_2 v_2 + x_3 v_3 < \text{Eps} \sqrt{x_1^2 + x_2^2 + x_3^2} \ \parallel \right. \\ \left. x_1 v_1 + x_2 v_2 + x_3 v_3 \leq 0 \right)$$

\$Aborted

$$\{3, x_1 < 0 \ \&\& \ x_2 > 0 \ \&\& \ x_3 == 0 \ \&\& \ x_4 < 0 \ \&\& \ x_5 == -\sqrt{\frac{x_1^2 x_4^2}{x_1^2 + x_2^2}} \ \&\& \ x_6 == \sqrt{x_4^2 - x_5^2}\}$$

$$\forall_{Eps, Eps > 0} \exists_{del, del > 0} \forall_{\{x_1, x_2, x_4\}, x_1 < 0 \&\& x_2 > 0 \&\& x_4 < 0 \&\& \sqrt{x_1^2 + x_2^2 + 2 x_4^2} < del} \left( -g_1 \sqrt{\frac{x_1^2 x_4^2}{x_1^2 + x_2^2}} + \right. \\ \left. g_2 \sqrt{x_4^2 - \frac{x_1^2 x_4^2}{x_1^2 + x_2^2}} + x_4 V + x_1 v_1 + x_2 v_2 < Eps \sqrt{x_1^2 + x_2^2 + 2 x_4^2} \parallel \right. \\ \left. -g_1 \sqrt{\frac{x_1^2 x_4^2}{x_1^2 + x_2^2}} + g_2 \sqrt{x_4^2 - \frac{x_1^2 x_4^2}{x_1^2 + x_2^2}} + x_4 V + x_1 v_1 + x_2 v_2 \leq 0 \right)$$

§Aborted

{4, x1 < 0 && x2 > 0 && x3 == 0 && x4 == 0 && x5 == 0 && x6 == 0}

$$\forall_{Eps, Eps > 0} \exists_{del, del > 0} \forall_{\{x_1, x_2\}, x_1 < 0 \&\& x_2 > 0 \&\& \sqrt{x_1^2 + x_2^2} < del} \left( x_1 v_1 + x_2 v_2 < Eps \sqrt{x_1^2 + x_2^2} \parallel x_1 v_1 + x_2 v_2 \leq 0 \right)$$

{0.800509, v2 ≤ 0 && v1 ≥ 0}

{5, x1 < 0 && x2 > 0 && x3 > 0 && x4 == 0 && x5 == 0 && x6 == 0}

$$\forall_{Eps, Eps > 0} \exists_{del, del > 0} \forall_{\{x_1, x_2, x_3\}, x_1 < 0 \&\& x_2 > 0 \&\& x_3 > 0 \&\& \sqrt{x_1^2 + x_2^2 + x_3^2} < del} \left( x_1 v_1 + x_2 v_2 + x_3 v_3 < Eps \sqrt{x_1^2 + x_2^2 + x_3^2} \parallel \right. \\ \left. x_1 v_1 + x_2 v_2 + x_3 v_3 \leq 0 \right)$$

§Aborted

{6, x1 == 0 && x2 < 0 && x3 == 0 && x4 ≤ 0 && x5 == 0 && x6 == -√x4^2}

$$\forall_{Eps, Eps > 0} \exists_{del, del > 0} \forall_{\{x_2, x_4\}, x_2 < 0 \&\& x_4 \leq 0 \&\& \sqrt{x_2^2 + 2 x_4^2} < del} \left( -g_2 \sqrt{x_4^2} + x_4 V + x_2 v_2 < Eps \sqrt{x_2^2 + 2 x_4^2} \parallel \right. \\ \left. -g_2 \sqrt{x_4^2} + x_4 V + x_2 v_2 \leq 0 \right)$$

§Aborted

{7, x1 == 0 && x2 < 0 && x3 > 0 && x4 == 0 && x5 == 0 && x6 == 0}

$$\forall_{Eps, Eps > 0} \exists_{del, del > 0} \forall_{\{x_2, x_3\}, x_2 < 0 \&\& x_3 > 0 \&\& \sqrt{x_2^2 + x_3^2} < del} \left( x_2 v_2 + x_3 v_3 < Eps \sqrt{x_2^2 + x_3^2} \parallel x_2 v_2 + x_3 v_3 \leq 0 \right)$$

{0.779923, v3 ≤ 0 && v2 ≥ 0}

{8, x1 == 0 && x2 == 0 && x3 == 0 && x4 < 0 && x5 == x4 && x6 == -√x4^2 - x5^2}

$$\forall_{Eps, Eps > 0} \exists_{del, del > 0} \forall_{\{x_4\}, x_4 < 0 \&\& \sqrt{2} \sqrt{x_4^2} < del} \left( g_1 x_4 + x_4 V < \sqrt{2} Eps \sqrt{x_4^2} \parallel g_1 x_4 + x_4 V \leq 0 \right)$$

{0.022001, g1 ≥ -V}

{9, x1 == 0 && x2 == 0 && x3 == 0 && x4 < 0 && x4 < x5 < -x4 && -√x4^2 - x5^2 ≤ x6 ≤ √x4^2 - x5^2}

$$\forall_{Eps, Eps > 0} \exists_{del, del > 0} \forall_{\{x_4, x_5, x_6\}, x_4 < 0 \&\& x_4 < x_5 < -x_4 \&\& -\sqrt{x_4^2 - x_5^2} \leq x_6 \leq \sqrt{x_4^2 - x_5^2} \&\& \sqrt{x_4^2 + x_5^2 + x_6^2} < del} \left( g_1 x_5 + g_2 x_6 + x_4 V < \right. \\ \left. Eps \sqrt{x_4^2 + x_5^2 + x_6^2} \parallel g_1 x_5 + g_2 x_6 + x_4 V \leq 0 \right)$$

§Aborted

{10, x1 == 0 && x2 == 0 && x3 == 0 && x4 < 0 && x5 == -x4 && x6 == -√x4^2 - x5^2}

$$\forall_{Eps, Eps > 0} \exists_{del, del > 0} \forall_{\{x_4\}, x_4 < 0 \&\& \sqrt{2} \sqrt{x_4^2} < del} \left( -g_1 x_4 + x_4 V < \sqrt{2} Eps \sqrt{x_4^2} \parallel -g_1 x_4 + x_4 V \leq 0 \right)$$

{0.022044, g1 ≤ V}

{11, x1 == 0 && x2 == 0 && x3 == 0 && x4 == 0 && x5 == 0 && x6 == 0}

$\forall_{\text{Eps}, \text{Eps} > 0} \exists_{\text{del}} \text{del} > 0$

{0.001949, True}

{12, x1 == 0 && x2 == 0 && x3 > 0 && x4 == 0 && x5 == 0 && x6 == 0}

$\forall_{\text{Eps}, \text{Eps} > 0} \exists_{\text{del}, \text{del} > 0} \forall_{\{x3\}, x3 > 0 \&\& \sqrt{x3^2} < \text{del}} \left( x3 v3 < \text{Eps} \sqrt{x3^2} \parallel x3 v3 \leq 0 \right)$

{0.013455, v3 ≤ 0}

{13, x1 == 0 && x2 > 0 && x3 == 0 && x4 < 0 && x5 == 0 && x6 ==  $\sqrt{x4^2}$ }

$\forall_{\text{Eps}, \text{Eps} > 0} \exists_{\text{del}, \text{del} > 0} \forall_{\{x2, x4\}, x2 > 0 \&\& x4 < 0 \&\& \sqrt{x2^2 + 2 x4^2} < \text{del}} \left( g2 \sqrt{x4^2} + x4 v + x2 v2 < \text{Eps} \sqrt{x2^2 + 2 x4^2} \parallel g2 \sqrt{x4^2} + x4 v + x2 v2 \leq 0 \right)$

\$Aborted

{14, x1 == 0 && x2 > 0 && x3 == 0 && x4 == 0 && x5 == 0 && x6 == 0}

$\forall_{\text{Eps}, \text{Eps} > 0} \exists_{\text{del}, \text{del} > 0} \forall_{\{x2\}, x2 > 0 \&\& \sqrt{x2^2} < \text{del}} \left( x2 v2 < \text{Eps} \sqrt{x2^2} \parallel x2 v2 \leq 0 \right)$

{0.01375, v2 ≤ 0}

{15, x1 == 0 && x2 > 0 && x3 > 0 && x4 == 0 && x5 == 0 && x6 == 0}

$\forall_{\text{Eps}, \text{Eps} > 0} \exists_{\text{del}, \text{del} > 0} \forall_{\{x2, x3\}, x2 > 0 \&\& x3 > 0 \&\& \sqrt{x2^2 + x3^2} < \text{del}} \left( x2 v2 + x3 v3 < \text{Eps} \sqrt{x2^2 + x3^2} \parallel x2 v2 + x3 v3 \leq 0 \right)$

{0.754768, v3 ≤ 0 && v2 ≤ 0}

{16, x1 > 0 && x2 < 0 && x3 == 0 && x4 ≤ 0 && x5 ==  $\sqrt{\frac{x1^2 x4^2}{x1^2 + x2^2}}$  && x6 ==  $-\sqrt{x4^2 - x5^2}$ }

$\forall_{\text{Eps}, \text{Eps} > 0} \exists_{\text{del}, \text{del} > 0} \forall_{\{x1, x2, x4\}, x1 > 0 \&\& x2 < 0 \&\& x4 \leq 0 \&\& \sqrt{x1^2 + x2^2 + 2 x4^2} < \text{del}} \left( g1 \sqrt{\frac{x1^2 x4^2}{x1^2 + x2^2}} - g2 \sqrt{x4^2 - \frac{x1^2 x4^2}{x1^2 + x2^2}} + x4 v + x1 v1 + x2 v2 < \text{Eps} \sqrt{x1^2 + x2^2 + 2 x4^2} \parallel g1 \sqrt{\frac{x1^2 x4^2}{x1^2 + x2^2}} - g2 \sqrt{x4^2 - \frac{x1^2 x4^2}{x1^2 + x2^2}} + x4 v + x1 v1 + x2 v2 \leq 0 \right)$

\$Aborted

{17, x1 > 0 && x2 < 0 && x3 > 0 && x4 == 0 && x5 == 0 && x6 == 0}

$\forall_{\text{Eps}, \text{Eps} > 0} \exists_{\text{del}, \text{del} > 0} \forall_{\{x1, x2, x3\}, x1 > 0 \&\& x2 < 0 \&\& x3 > 0 \&\& \sqrt{x1^2 + x2^2 + x3^2} < \text{del}} \left( x1 v1 + x2 v2 + x3 v3 < \text{Eps} \sqrt{x1^2 + x2^2 + x3^2} \parallel x1 v1 + x2 v2 + x3 v3 \leq 0 \right)$

\$Aborted

{18, x1 > 0 && x2 == 0 && x3 == 0 && x4 ≤ 0 && x5 ==  $-x4$  && x6 ==  $-\sqrt{x4^2 - x5^2}$ }

$$\forall_{\text{Eps}, \text{Eps} > 0} \exists_{\text{del}, \text{del} > 0} \forall_{\{x_1, x_4\}, x_1 > 0 \&\& x_4 \leq 0 \&\& \sqrt{x_1^2 + 2x_4^2} < \text{del}} \left( -g_1 x_4 + x_4 V + x_1 v_1 < \text{Eps} \sqrt{x_1^2 + 2x_4^2} \parallel \right. \\ \left. -g_1 x_4 + x_4 V + x_1 v_1 \leq 0 \right)$$

$$\{0.794348, g_1 \leq V \&\& v_1 \leq 0\}$$

$$\{19, x_1 > 0 \&\& x_2 == 0 \&\& x_3 > 0 \&\& x_4 == 0 \&\& x_5 == 0 \&\& x_6 == 0\}$$

$$\forall_{\text{Eps}, \text{Eps} > 0} \exists_{\text{del}, \text{del} > 0} \forall_{\{x_1, x_3\}, x_1 > 0 \&\& x_3 > 0 \&\& \sqrt{x_1^2 + x_3^2} < \text{del}} \left( x_1 v_1 + x_3 v_3 < \text{Eps} \sqrt{x_1^2 + x_3^2} \parallel x_1 v_1 + x_3 v_3 \leq 0 \right)$$

$$\{0.531973, v_3 \leq 0 \&\& v_1 \leq 0\}$$

$$\{20, x_1 > 0 \&\& x_2 > 0 \&\& x_3 == 0 \&\& x_4 < 0 \&\& x_5 == \sqrt{\frac{x_1^2 x_4^2}{x_1^2 + x_2^2}} \&\& x_6 == \sqrt{x_4^2 - x_5^2}\}$$

$$\forall_{\text{Eps}, \text{Eps} > 0} \exists_{\text{del}, \text{del} > 0} \forall_{\{x_1, x_2, x_4\}, x_1 > 0 \&\& x_2 > 0 \&\& x_4 < 0 \&\& \sqrt{x_1^2 + x_2^2 + 2x_4^2} < \text{del}} \left( g_1 \sqrt{\frac{x_1^2 x_4^2}{x_1^2 + x_2^2}} + \right. \\ \left. g_2 \sqrt{x_4^2 - \frac{x_1^2 x_4^2}{x_1^2 + x_2^2}} + x_4 V + x_1 v_1 + x_2 v_2 < \text{Eps} \sqrt{x_1^2 + x_2^2 + 2x_4^2} \parallel \right. \\ \left. g_1 \sqrt{\frac{x_1^2 x_4^2}{x_1^2 + x_2^2}} + g_2 \sqrt{x_4^2 - \frac{x_1^2 x_4^2}{x_1^2 + x_2^2}} + x_4 V + x_1 v_1 + x_2 v_2 \leq 0 \right)$$

\$Aborted

$$\{21, x_1 > 0 \&\& x_2 > 0 \&\& x_3 == 0 \&\& x_4 == 0 \&\& x_5 == 0 \&\& x_6 == 0\}$$

$$\forall_{\text{Eps}, \text{Eps} > 0} \exists_{\text{del}, \text{del} > 0} \forall_{\{x_1, x_2\}, x_1 > 0 \&\& x_2 > 0 \&\& \sqrt{x_1^2 + x_2^2} < \text{del}} \left( x_1 v_1 + x_2 v_2 < \text{Eps} \sqrt{x_1^2 + x_2^2} \parallel x_1 v_1 + x_2 v_2 \leq 0 \right)$$

$$\{0.758715, v_2 \leq 0 \&\& v_1 \leq 0\}$$

$$\{22, x_1 > 0 \&\& x_2 > 0 \&\& x_3 > 0 \&\& x_4 == 0 \&\& x_5 == 0 \&\& x_6 == 0\}$$

$$\forall_{\text{Eps}, \text{Eps} > 0} \exists_{\text{del}, \text{del} > 0} \forall_{\{x_1, x_2, x_3\}, x_1 > 0 \&\& x_2 > 0 \&\& x_3 > 0 \&\& \sqrt{x_1^2 + x_2^2 + x_3^2} < \text{del}} \left( x_1 v_1 + x_2 v_2 + x_3 v_3 < \text{Eps} \sqrt{x_1^2 + x_2^2 + x_3^2} \parallel \right. \\ \left. x_1 v_1 + x_2 v_2 + x_3 v_3 \leq 0 \right)$$

\$Aborted

In[56]:= **res**

Out[56]=

$$\{v_2 \leq 0 \&\& v_1 \geq 0, v_3 \leq 0 \&\& v_2 \geq 0, g_1 \geq -V, g_1 \leq V, \text{True}, v_3 \leq 0, \\ v_2 \leq 0, v_3 \leq 0 \&\& v_2 \leq 0, g_1 \leq V \&\& v_1 \leq 0, v_3 \leq 0 \&\& v_1 \leq 0, v_2 \leq 0 \&\& v_1 \leq 0\}$$

(\* Conditions found for v\*'s after the first run. \*)

In[57]:= **Simplify[And@@res]**

Out[57]=

$$g_1 + V \geq 0 \&\& v_1 == 0 \&\& v_2 == 0 \&\& g_1 \leq V \&\& v_3 \leq 0$$

(\* Indices of cells we couldn't finish the calculations of after the first run: \*)

In[58]:= **ind**

Out[58]=

{1, 2, 3, 5, 6, 9, 13, 16, 17, 20, 22}

There are some cases that are obviously solvable but Mathematica failed because it doesn't simplify square roots fully:

### Case 6 done by hand

In[59]:= **splt[GphCADSim[6]]**(\* The innermost clause has  $x_4 \leq 0$ ,  
therefore we can conclude that  $\sqrt{x_4^2} == -x_4$ . \*)

Out[59]=

$$\forall \text{Eps}, \text{Eps} > 0 \exists \text{del}, \text{del} > 0 \forall_{\{x_2, x_4\}, x_2 < 0 \&\& x_4 \leq 0 \&\& \sqrt{x_2^2 + 2 x_4^2} < \text{del}} \left( -g_2 \sqrt{x_4^2} + x_4 V + x_2 v_2 < \text{Eps} \sqrt{x_2^2 + 2 x_4^2} \parallel \right. \\ \left. -g_2 \sqrt{x_4^2} + x_4 V + x_2 v_2 \leq 0 \right)$$

In[60]:= **Timing[Reduce[splt[GphCADSim[6]] /.  $\sqrt{x_4^2} \rightarrow -x_4$ ]]**

Out[60]=

{1.27728,  $V \in \mathbb{R} \&\& g_2 \geq -V \&\& v_2 \geq 0$ }

(\* Delete case 6 from unsolved cases \*)

In[61]:= **ind**

Out[61]=

{1, 2, 3, 5, 6, 9, 13, 16, 17, 20, 22}

In[62]:= **ind = Delete[ind, FirstPosition[ind, 6]]**

Out[62]=

{1, 2, 3, 5, 9, 13, 16, 17, 20, 22}

In[63]:= **ind**

Out[63]=

{1, 2, 3, 5, 9, 13, 16, 17, 20, 22}

### Case 13 done by hand

In[64]:= **splt[GphCADSim[13]]**(\* The innermost clause has  $x_4 < 0$ ,  
therefore we can conclude that  $\sqrt{x_4^2} == -x_4$ . \*)

Out[64]=

$$\forall \text{Eps}, \text{Eps} > 0 \exists \text{del}, \text{del} > 0 \forall_{\{x_2, x_4\}, x_2 > 0 \&\& x_4 < 0 \&\& \sqrt{x_2^2 + 2 x_4^2} < \text{del}} \left( g_2 \sqrt{x_4^2} + x_4 V + x_2 v_2 < \text{Eps} \sqrt{x_2^2 + 2 x_4^2} \parallel \right. \\ \left. g_2 \sqrt{x_4^2} + x_4 V + x_2 v_2 \leq 0 \right)$$

```
In[65]:= Timing[Reduce[splt[GphCADSim[13]] /.  $\sqrt{x^4} \rightarrow -x^4$ ]]
```

```
Out[65]= {1.14271, V ∈ ℝ && g2 ≤ V && v2 ≤ 0}
```

```
(* Delete case 13 from unsolx4ed cases *)
```

```
In[66]:= ind
```

```
Out[66]= {1, 2, 3, 5, 9, 13, 16, 17, 20, 22}
```

```
In[67]:= ind = Delete[ind, FirstPosition[ind, 13]]
```

```
Out[67]= {1, 2, 3, 5, 9, 16, 17, 20, 22}
```

```
In[68]:= ind
```

```
Out[68]= {1, 2, 3, 5, 9, 16, 17, 20, 22}
```

## Add the hand solved conditions to the pool of conditions on the normal cone N\_C

```
In[69]:= res
```

```
Out[69]= {v2 ≤ 0 && v1 ≥ 0, v3 ≤ 0 && v2 ≥ 0, g1 ≥ -V, g1 ≤ V, True, v3 ≤ 0,
v2 ≤ 0, v3 ≤ 0 && v2 ≤ 0, g1 ≤ V && v1 ≤ 0, v3 ≤ 0 && v1 ≤ 0, v2 ≤ 0 && v1 ≤ 0}
```

```
In[70]:= AppendTo[res, g2 ∈ ℝ && V ≥ -g2 && v2 ≥ 0] (* add solution of case 6 to the pool *)
```

```
Out[70]= {v2 ≤ 0 && v1 ≥ 0, v3 ≤ 0 && v2 ≥ 0, g1 ≥ -V, g1 ≤ V, True, v3 ≤ 0, v2 ≤ 0, v3 ≤ 0 && v2 ≤ 0,
g1 ≤ V && v1 ≤ 0, v3 ≤ 0 && v1 ≤ 0, v2 ≤ 0 && v1 ≤ 0, g2 ∈ ℝ && V ≥ -g2 && v2 ≥ 0}
```

```
In[71]:= AppendTo[res, g2 ∈ ℝ && V ≥ g2 && v2 ≤ 0] (* add solution of case 13 to the pool *)
```

```
Out[71]= {v2 ≤ 0 && v1 ≥ 0, v3 ≤ 0 && v2 ≥ 0, g1 ≥ -V, g1 ≤ V, True,
v3 ≤ 0, v2 ≤ 0, v3 ≤ 0 && v2 ≤ 0, g1 ≤ V && v1 ≤ 0, v3 ≤ 0 && v1 ≤ 0,
v2 ≤ 0 && v1 ≤ 0, g2 ∈ ℝ && V ≥ -g2 && v2 ≥ 0, g2 ∈ ℝ && V ≥ g2 && v2 ≤ 0}
```

```
(* Conditions on v*'s after resolving the two cells by hand. *)
```

```
In[72]:= Simplify[And@@res]
```

```
Out[72]= g2 ∈ ℝ && g1 + V ≥ 0 && g2 + V ≥ 0 && g2 ≤ V && v1 == 0 && v2 == 0 && g1 ≤ V && v3 ≤ 0
```

## Update N\_i (i.e. CAD of the overestimates of the normal cone for gph(Q))

```
In[73]:= Ni = CylindricalDecomposition[And@@res, {v1, v2, v3, V, g1, g2}]
```

```
Out[73]= v1 == 0 && v2 == 0 && v3 ≤ 0 && ((V == 0 && g1 == 0 && g2 == 0) || (V > 0 && -V ≤ g1 ≤ V && -V ≤ g2 ≤ V))
```

(\* The semialgebraic description above is the same as the following: \*)

```
In[74]:= Ni = v1 == 0 && v2 == 0 && v3 ≤ 0 && V ≥ 0 && -V ≤ g1 ≤ V && -V ≤ g2 ≤ V;
```

We learned that  $v1 == v2 == 0$  in  $Ni$ . Therefore, we can use these substitutions and attempt QE on the previously failed cells :

```
In[75]:= ind(* unsolved cases of GphCADSim - the DNF CAD of the graph. *)
```

```
Out[75]=
```

```
{1, 2, 3, 5, 9, 16, 17, 20, 22}
```

(\* Run QE on the unsolved cases with the extra knowledge that  $v1==v2==0$ . \*)

```
In[76]:= T = 1;
```

```
ind2 = {}; (* List of unsolved cases *)
```

```
Do[
```

```
  tres = $Aborted;
```

```
  Print[Style[{ind[i]}, GphCADSim[ind[i]]], Red];
```

```
  (* Prints the index and the description of the combined cell*)
```

```
  Print[Style[Simplify[splt[GphCADSim[ind[i]]] /. {v1 → 0, v2 → 0}], Blue];
```

```
  (* Prints the Normal cone definition structure QE needs to solve*)
```

```
  (* Here we impose v1==v2==0 too *)
```

```
  Print[TimeConstrained[
```

```
    Timing[tres = Resolve[splt[GphCADSim[ind[i]]] /. {v1 → 0, v2 → 0}, Reals], T];
```

```
  (*Tries QE and prints the outcome *)
```

```
  If[tres != $Aborted, AppendTo[res, tres], AppendTo[ind2, ind[i]]]
```

```
  (*If the calculation yielded a solution,
```

```
  records this in res, add indices of failed cells to ind2*)
```

```
,
```

```
{i, 1, Length[ind]}]
```

$$\left\{1, x1 < 0 \ \&\& \ x2 \leq 0 \ \&\& \ x3 == 0 \ \&\& \ x4 \leq 0 \ \&\& \ x5 == -\sqrt{\frac{x1^2 x4^2}{x1^2 + x2^2}} \ \&\& \ x6 == -\sqrt{x4^2 - x5^2}\right\}$$

$$\forall_{Eps, Eps > 0} \exists_{del, del > 0} \forall_{(x1, x2, x4), x1 < 0 \ \&\& \ x2 \leq 0 \ \&\& \ x4 \leq 0 \ \&\& \ \sqrt{x1^2 + x2^2 + 2 x4^2} < del \left( -g1 \sqrt{\frac{x1^2 x4^2}{x1^2 + x2^2}} - g2 \sqrt{x4^2 - \frac{x1^2 x4^2}{x1^2 + x2^2}} + x4 V <$$

$$Eps \sqrt{x1^2 + x2^2 + 2 x4^2} \parallel -g1 \sqrt{\frac{x1^2 x4^2}{x1^2 + x2^2}} - g2 \sqrt{x4^2 - \frac{x1^2 x4^2}{x1^2 + x2^2}} + x4 V \leq 0 \right)$$

```
$Aborted
```

```
{2, x1 < 0 && x2 ≤ 0 && x3 > 0 && x4 == 0 && x5 == 0 && x6 == 0}
```

```
 $\forall_{Eps, Eps > 0} \exists_{del, del > 0} \forall_{(x1, x2, x3), x1 < 0 \ \&\& \ x2 \leq 0 \ \&\& \ x3 > 0 \ \&\& \ \sqrt{x1^2 + x2^2 + x3^2} < del \left( x3 v3 < Eps \sqrt{x1^2 + x2^2 + x3^2} \parallel x3 v3 \leq 0 \right)$ 
```

```
{0.038425, v3 ≤ 0}
```

$$\{3, x1 < 0 \ \&\& \ x2 > 0 \ \&\& \ x3 == 0 \ \&\& \ x4 < 0 \ \&\& \ x5 == -\sqrt{\frac{x1^2 x4^2}{x1^2 + x2^2}} \ \&\& \ x6 == \sqrt{x4^2 - x5^2}\}$$

$$\forall_{\text{Eps}, \text{Eps} > 0} \exists_{\text{del}, \text{del} > 0} \forall_{\{x1, x2, x4\}, x1 < 0 \ \&\& \ x2 > 0 \ \&\& \ x4 < 0 \ \&\& \ \sqrt{x1^2 + x2^2 + 2 x4^2} < \text{del}} \left( -g1 \sqrt{\frac{x1^2 x4^2}{x1^2 + x2^2}} + g2 \sqrt{x4^2 - \frac{x1^2 x4^2}{x1^2 + x2^2}} + x4 V < \right. \\ \left. \text{Eps} \sqrt{x1^2 + x2^2 + 2 x4^2} \ \parallel -g1 \sqrt{\frac{x1^2 x4^2}{x1^2 + x2^2}} + g2 \sqrt{x4^2 - \frac{x1^2 x4^2}{x1^2 + x2^2}} + x4 V \leq 0 \right)$$

§Aborted

$$\{5, x1 < 0 \ \&\& \ x2 > 0 \ \&\& \ x3 > 0 \ \&\& \ x4 == 0 \ \&\& \ x5 == 0 \ \&\& \ x6 == 0\}$$

$$\forall_{\text{Eps}, \text{Eps} > 0} \exists_{\text{del}, \text{del} > 0} \forall_{\{x1, x2, x3\}, x1 < 0 \ \&\& \ x2 > 0 \ \&\& \ x3 > 0 \ \&\& \ \sqrt{x1^2 + x2^2 + x3^2} < \text{del}} \left( x3 v3 < \text{Eps} \sqrt{x1^2 + x2^2 + x3^2} \ \parallel x3 v3 \leq 0 \right)$$

$$\{0.034609, v3 \leq 0\}$$

$$\{9, x1 == 0 \ \&\& \ x2 == 0 \ \&\& \ x3 == 0 \ \&\& \ x4 < 0 \ \&\& \ x4 < x5 < -x4 \ \&\& \ -\sqrt{x4^2 - x5^2} \leq x6 \leq \sqrt{x4^2 - x5^2}\}$$

$$\forall_{\text{Eps}, \text{Eps} > 0} \exists_{\text{del}, \text{del} > 0} \forall_{\{x4, x5, x6\}, x4 < 0 \ \&\& \ x4 < x5 < -x4 \ \&\& \ -\sqrt{x4^2 - x5^2} \leq x6 \leq \sqrt{x4^2 - x5^2} \ \&\& \ \sqrt{x4^2 + x5^2 + x6^2} < \text{del}} \left( g1 x5 + g2 x6 + x4 V < \right. \\ \left. \text{Eps} \sqrt{x4^2 + x5^2 + x6^2} \ \parallel g1 x5 + g2 x6 + x4 V \leq 0 \right)$$

§Aborted

$$\{16, x1 > 0 \ \&\& \ x2 < 0 \ \&\& \ x3 == 0 \ \&\& \ x4 \leq 0 \ \&\& \ x5 == \sqrt{\frac{x1^2 x4^2}{x1^2 + x2^2}} \ \&\& \ x6 == -\sqrt{x4^2 - x5^2}\}$$

$$\forall_{\text{Eps}, \text{Eps} > 0} \exists_{\text{del}, \text{del} > 0} \forall_{\{x1, x2, x4\}, x1 > 0 \ \&\& \ x2 < 0 \ \&\& \ x4 \leq 0 \ \&\& \ \sqrt{x1^2 + x2^2 + 2 x4^2} < \text{del}} \left( g1 \sqrt{\frac{x1^2 x4^2}{x1^2 + x2^2}} - g2 \sqrt{x4^2 - \frac{x1^2 x4^2}{x1^2 + x2^2}} + x4 V < \right. \\ \left. \text{Eps} \sqrt{x1^2 + x2^2 + 2 x4^2} \ \parallel g1 \sqrt{\frac{x1^2 x4^2}{x1^2 + x2^2}} - g2 \sqrt{x4^2 - \frac{x1^2 x4^2}{x1^2 + x2^2}} + x4 V \leq 0 \right)$$

§Aborted

$$\{17, x1 > 0 \ \&\& \ x2 < 0 \ \&\& \ x3 > 0 \ \&\& \ x4 == 0 \ \&\& \ x5 == 0 \ \&\& \ x6 == 0\}$$

$$\forall_{\text{Eps}, \text{Eps} > 0} \exists_{\text{del}, \text{del} > 0} \forall_{\{x1, x2, x3\}, x1 > 0 \ \&\& \ x2 < 0 \ \&\& \ x3 > 0 \ \&\& \ \sqrt{x1^2 + x2^2 + x3^2} < \text{del}} \left( x3 v3 < \text{Eps} \sqrt{x1^2 + x2^2 + x3^2} \ \parallel x3 v3 \leq 0 \right)$$

$$\{0.039922, v3 \leq 0\}$$

$$\{20, x1 > 0 \ \&\& \ x2 > 0 \ \&\& \ x3 == 0 \ \&\& \ x4 < 0 \ \&\& \ x5 == \sqrt{\frac{x1^2 x4^2}{x1^2 + x2^2}} \ \&\& \ x6 == \sqrt{x4^2 - x5^2}\}$$

$$\forall_{\text{Eps}, \text{Eps} > 0} \exists_{\text{del}, \text{del} > 0} \forall_{\{x1, x2, x4\}, x1 > 0 \ \&\& \ x2 > 0 \ \&\& \ x4 < 0 \ \&\& \ \sqrt{x1^2 + x2^2 + 2 x4^2} < \text{del}} \left( g1 \sqrt{\frac{x1^2 x4^2}{x1^2 + x2^2}} + g2 \sqrt{x4^2 - \frac{x1^2 x4^2}{x1^2 + x2^2}} + x4 V < \right. \\ \left. \text{Eps} \sqrt{x1^2 + x2^2 + 2 x4^2} \ \parallel g1 \sqrt{\frac{x1^2 x4^2}{x1^2 + x2^2}} + g2 \sqrt{x4^2 - \frac{x1^2 x4^2}{x1^2 + x2^2}} + x4 V \leq 0 \right)$$

§Aborted

```
{22, x1 > 0 && x2 > 0 && x3 > 0 && x4 == 0 && x5 == 0 && x6 == 0}
```

```
 $\forall_{\text{Eps}, \text{Eps} > 0} \exists_{\text{del}, \text{del} > 0} \forall_{\{x_1, x_2, x_3, x_1 > 0 \&\& x_2 > 0 \&\& x_3 > 0 \&\& \sqrt{x_1^2 + x_2^2 + x_3^2} < \text{del}\}} (x_3 v_3 < \text{Eps} \sqrt{x_1^2 + x_2^2 + x_3^2} \parallel x_3 v_3 \leq 0)$ 
```

```
{0.029381, v3 ≤ 0}
```

```
(* Updated list of conditions*)
```

```
In[79]:= res
```

```
Out[79]=
```

```
{v2 ≤ 0 && v1 ≥ 0, v3 ≤ 0 && v2 ≥ 0, g1 ≥ -V, g1 ≤ V, True, v3 ≤ 0,
 v2 ≤ 0, v3 ≤ 0 && v2 ≤ 0, g1 ≤ V && v1 ≤ 0, v3 ≤ 0 && v1 ≤ 0, v2 ≤ 0 && v1 ≤ 0,
 g2 ∈ ℝ && V ≥ -g2 && v2 ≥ 0, g2 ∈ ℝ && V ≥ g2 && v2 ≤ 0, v3 ≤ 0, v3 ≤ 0, v3 ≤ 0, v3 ≤ 0}
```

```
(* Checking if,
```

```
the normal cone upper estimate is the same after adding these new conditions: *)
```

```
In[80]:= Reduce[Not[(And @@ res)] && Ni]
```

```
Out[80]=
```

```
False
```

```
(* We have not found any point that is inside the upper estimate we already found
 that is outside of the new refined upper estimate. Therefore they are the same.*)
```

```
In[81]:= (* The unresolved Cell numbers: *)
```

```
ind2
```

```
Out[81]=
```

```
{1, 3, 9, 16, 20}
```

Cases 1, 3, 16, and 20 are similar and they fail because of the square-root/rational function simplifications:

```
In[82]:= GphCADSim[1]
```

```
Out[82]=
```

$$x_1 < 0 \&\& x_2 \leq 0 \&\& x_3 == 0 \&\& x_4 \leq 0 \&\& x_5 == -\sqrt{\frac{x_1^2 x_4^2}{x_1^2 + x_2^2}} \&\& x_6 == -\sqrt{x_4^2 - x_5^2}$$

```
In[83]:= GphCADSim[3]
```

```
Out[83]=
```

$$x_1 < 0 \&\& x_2 > 0 \&\& x_3 == 0 \&\& x_4 < 0 \&\& x_5 == -\sqrt{\frac{x_1^2 x_4^2}{x_1^2 + x_2^2}} \&\& x_6 == \sqrt{x_4^2 - x_5^2}$$

```
In[84]:= GphCADSim[16]
```

```
Out[84]=
```

$$x_1 > 0 \&\& x_2 < 0 \&\& x_3 == 0 \&\& x_4 \leq 0 \&\& x_5 == \sqrt{\frac{x_1^2 x_4^2}{x_1^2 + x_2^2}} \&\& x_6 == -\sqrt{x_4^2 - x_5^2}$$

In[85]:= **GphCADSim**[[20]]

Out[85]=

$$x1 > 0 \ \&\& \ x2 > 0 \ \&\& \ x3 == 0 \ \&\& \ x4 < 0 \ \&\& \ x5 == \sqrt{\frac{x1^2 x4^2}{x1^2 + x2^2}} \ \&\& \ x6 == \sqrt{x4^2 - x5^2}$$

**Observation:** Cases 1, 3, 16, and 20 combined gives the conditions  $x1 \neq 0 \ || \ x2 \neq 0$ .  
With that in mind, we can simplify denominators, etc. to make it easier for the solver.

### Case 1: (read comment inside)

In[86]:= **splt**[**GphCADSim**[[1]]]

Out[86]=

$$\forall_{Eps, Eps > 0} \exists_{del, del > 0} \forall_{\{x1, x2, x4\}, x1 < 0 \ \&\& \ x2 \leq 0 \ \&\& \ x4 \leq 0 \ \&\& \ \sqrt{x1^2 + x2^2 + 2 x4^2} < del} \left( -g1 \sqrt{\frac{x1^2 x4^2}{x1^2 + x2^2}} - \right. \\ \left. g2 \sqrt{x4^2 - \frac{x1^2 x4^2}{x1^2 + x2^2}} + x4 V + x1 v1 + x2 v2 < Eps \sqrt{x1^2 + x2^2 + 2 x4^2} \ || \right. \\ \left. -g1 \sqrt{\frac{x1^2 x4^2}{x1^2 + x2^2}} - g2 \sqrt{x4^2 - \frac{x1^2 x4^2}{x1^2 + x2^2}} + x4 V + x1 v1 + x2 v2 \leq 0 \right)$$

In[87]:= **Reduce** `ToPrenexForm

$$\forall_{\{x1, x2, x4\}, x1 < 0 \ \&\& \ x2 \leq 0 \ \&\& \ x4 \leq 0 \ \&\& \ \sqrt{x1^2 + x2^2 + 2 x4^2} < del} \left( -g1 \sqrt{\frac{x1^2 x4^2}{x1^2 + x2^2}} - g2 \sqrt{x4^2 - \frac{x1^2 x4^2}{x1^2 + x2^2}} + \right. \\ \left. x4 V + x1 v1 + x2 v2 < Eps \sqrt{x1^2 + x2^2 + 2 x4^2} \ || \right. \\ \left. -g1 \sqrt{\frac{x1^2 x4^2}{x1^2 + x2^2}} - g2 \sqrt{x4^2 - \frac{x1^2 x4^2}{x1^2 + x2^2}} + x4 V + x1 v1 + x2 v2 \leq 0 \right)$$

Out[87]=

$$\forall_{\{c1, c2, c3\}} \left( c1 \geq 0 \ || \ \sqrt{c1^2 + c2^2 + 2 c3^2} \geq del \ || \right. \\ \left. -g1 \sqrt{\frac{c1^2 c3^2}{c1^2 + c2^2}} - g2 \sqrt{c3^2 - \frac{c1^2 c3^2}{c1^2 + c2^2}} + c3 V + c1 v1 + c2 v2 < Eps \sqrt{c1^2 + c2^2 + 2 c3^2} \ || \right. \\ \left. c2 > 0 \ || \ c3 > 0 \ || -g1 \sqrt{\frac{c1^2 c3^2}{c1^2 + c2^2}} - g2 \sqrt{c3^2 - \frac{c1^2 c3^2}{c1^2 + c2^2}} + c3 V + c1 v1 + c2 v2 \leq 0 \right)$$

(\* When  $x_1(=e_1) \geq 0$  or  $x_2(=e_2) > 0$  or  $x_4(=e_3) > 0$  gets satisfied the whole thing is True, hence we do not get a restriction for  $N_i$ .

We need to solve this when  $x_1 < 0$ ,  $x_2 \leq 0$  and  $x_4 \geq 0$ .

This allows us to correctly simplify  $\text{Sqrt}[x_1^2]$  and  $\text{Sqrt}[x_2^2]$ .

We can also restrict our solutions within  $N_i$  to limit the search space. Furthermore, we can only use the  $V, g_1, g_2$  projection of  $N_i$  since the other variables do not even play a role in these calculations. \*)

In[88]:= **Ni**

Out[88]=

$v_1 == 0 \ \&\& \ v_2 == 0 \ \&\& \ v_3 \leq 0 \ \&\& \ V \geq 0 \ \&\& \ -V \leq g_1 \leq V \ \&\& \ -V \leq g_2 \leq V$

In[89]:=  $\forall \text{Eps}, \text{Eps} > 0 \ \exists \text{del}, \text{del} > 0 \ \forall_{\{x_1, x_2, x_4\}, x_1 < 0 \ \&\& \ x_2 \leq 0 \ \&\& \ x_4 \geq 0 \ \&\& \ \sqrt{x_1^2 + x_2^2 + 2 x_4^2} < \text{del}} \left( -g_1 \sqrt{\frac{x_1^2 x_4^2}{x_1^2 + x_2^2}} - \right.$   
 $g_2 \sqrt{x_4^2 - \frac{x_1^2 x_4^2}{x_1^2 + x_2^2}} + x_4 V + x_1 v_1 + x_2 v_2 < \text{Eps} \sqrt{x_1^2 + x_2^2 + 2 x_4^2} \ \parallel$   
 $\left. -g_1 \sqrt{\frac{x_1^2 x_4^2}{x_1^2 + x_2^2}} - g_2 \sqrt{x_4^2 - \frac{x_1^2 x_4^2}{x_1^2 + x_2^2}} + x_4 V + x_1 v_1 + x_2 v_2 \leq 0 \right)$

Out[89]=

$\forall \text{Eps}, \text{Eps} > 0 \ \exists \text{del}, \text{del} > 0 \ \forall_{\{x_1, x_2, x_4\}, x_1 < 0 \ \&\& \ x_2 \leq 0 \ \&\& \ x_4 \geq 0 \ \&\& \ \sqrt{x_1^2 + x_2^2 + 2 x_4^2} < \text{del}} \left( -g_1 \sqrt{\frac{x_1^2 x_4^2}{x_1^2 + x_2^2}} - \right.$   
 $g_2 \sqrt{x_4^2 - \frac{x_1^2 x_4^2}{x_1^2 + x_2^2}} + x_4 V + x_1 v_1 + x_2 v_2 < \text{Eps} \sqrt{x_1^2 + x_2^2 + 2 x_4^2} \ \parallel$   
 $\left. -g_1 \sqrt{\frac{x_1^2 x_4^2}{x_1^2 + x_2^2}} - g_2 \sqrt{x_4^2 - \frac{x_1^2 x_4^2}{x_1^2 + x_2^2}} + x_4 V + x_1 v_1 + x_2 v_2 \leq 0 \right)$

In[90]:= **Timing[Case1res = CylindricalDecomposition[**

**Ni &&  $x_1 < 0 \ \&\& \ x_2 \leq 0 \ \&\& \ x_4 \geq 0 \ \&\& \ (\forall \text{Eps}, \text{Eps} > 0 \ \exists \text{del}, \text{del} > 0 \ \text{Implies}[\sqrt{x_1^2 + x_2^2 + 2 x_4^2} < \text{del},$**   
 $-g_1 x_1 x_4 - g_2 x_2 x_4 + (x_4 V + x_1 v_1 + x_2 v_2) \sqrt{x_1^2 + x_2^2} < \text{Eps} \sqrt{x_1^2 + x_2^2} \sqrt{x_1^2 + x_2^2 + 2 x_4^2} \ \parallel$   
 $-g_1 x_1 x_4 - g_2 x_2 x_4 + (x_4 V + x_1 v_1 + x_2 v_2) \sqrt{x_1^2 + x_2^2} \leq 0]]),$   
 $\{x_1, x_2, x_4, v_1, v_2, v_3, V, g_2, g_1\}]$

Out[90]=

$\{224.46, x_1 < 0 \ \&\& \ x_2 \leq 0 \ \&\& \ x_4 \geq 0 \ \&\& \ v_1 == 0 \ \&\& \ v_2 == 0 \ \&\& \ v_3 \leq 0 \ \&\& \ (V == 0 \ \&\& \ g_2 == 0 \ \&\& \ g_1 == 0) \ \parallel \ (V > 0 \ \&\& \ -V \leq g_2 \leq V \ \&\& \ -V \leq g_1 \leq V)\}$

### Case 3:

In[91]:= `splt[GphCADSim[3]]`

Out[91]=

$$\forall_{\text{Eps}, \text{Eps} > 0} \exists_{\text{del}, \text{del} > 0} \forall_{\{x_1, x_2, x_4\}, x_1 < 0 \ \&\& \ x_2 > 0 \ \&\& \ x_4 < 0 \ \&\& \ \sqrt{x_1^2 + x_2^2 + 2 x_4^2} < \text{del}} \left( -g_1 \sqrt{\frac{x_1^2 x_4^2}{x_1^2 + x_2^2}} + \right. \\ \left. g_2 \sqrt{x_4^2 - \frac{x_1^2 x_4^2}{x_1^2 + x_2^2}} + x_4 V + x_1 v_1 + x_2 v_2 < \text{Eps} \sqrt{x_1^2 + x_2^2 + 2 x_4^2} \ \parallel \right. \\ \left. -g_1 \sqrt{\frac{x_1^2 x_4^2}{x_1^2 + x_2^2}} + g_2 \sqrt{x_4^2 - \frac{x_1^2 x_4^2}{x_1^2 + x_2^2}} + x_4 V + x_1 v_1 + x_2 v_2 \leq 0 \right)$$

In[92]:= `Timing[Case3res = CylindricalDecomposition[`

$$\text{Ni} \ \&\& \ x_1 < 0 \ \&\& \ x_2 > 0 \ \&\& \ x_4 < 0 \ \&\& \ \left( \forall_{\text{Eps}, \text{Eps} > 0} \exists_{\text{del}, \text{del} > 0} \text{Implies} \left[ \sqrt{x_1^2 + x_2^2 + 2 x_4^2} < \text{del}, \right. \right. \\ \left. \left. -g_1 x_1 x_4 - g_2 x_2 x_4 + (x_4 V + x_1 v_1 + x_2 v_2) \sqrt{x_1^2 + x_2^2} < \text{Eps} \sqrt{x_1^2 + x_2^2} \sqrt{x_1^2 + x_2^2 + 2 x_4^2} \ \parallel \right. \right. \\ \left. \left. -g_1 x_1 x_4 - g_2 x_2 x_4 + (x_4 V + x_1 v_1 + x_2 v_2) \sqrt{x_1^2 + x_2^2} \leq 0 \right] \right), \\ \left. \{x_1, x_2, x_4, v_1, v_2, v_3, V, g_2, g_1\} \right]$$

Out[92]=

$$\{210.856, x_1 < 0 \ \&\& \ x_2 > 0 \ \&\& \ x_4 < 0 \ \&\& \ v_1 == 0 \ \&\& \ v_2 == 0 \ \&\& \\ v_3 \leq 0 \ \&\& \ ((V == 0 \ \&\& \ g_2 == 0 \ \&\& \ g_1 == 0) \ \parallel \ (V > 0 \ \&\& \ -V \leq g_2 \leq V \ \&\& \ -V \leq g_1 \leq V))\}$$

### Case 16:

In[93]:= `splt[GphCADSim[16]]`

Out[93]=

$$\forall_{\text{Eps}, \text{Eps} > 0} \exists_{\text{del}, \text{del} > 0} \forall_{\{x_1, x_2, x_4\}, x_1 > 0 \ \&\& \ x_2 < 0 \ \&\& \ x_4 \leq 0 \ \&\& \ \sqrt{x_1^2 + x_2^2 + 2 x_4^2} < \text{del}} \left( g_1 \sqrt{\frac{x_1^2 x_4^2}{x_1^2 + x_2^2}} - \right. \\ \left. g_2 \sqrt{x_4^2 - \frac{x_1^2 x_4^2}{x_1^2 + x_2^2}} + x_4 V + x_1 v_1 + x_2 v_2 < \text{Eps} \sqrt{x_1^2 + x_2^2 + 2 x_4^2} \ \parallel \right. \\ \left. g_1 \sqrt{\frac{x_1^2 x_4^2}{x_1^2 + x_2^2}} - g_2 \sqrt{x_4^2 - \frac{x_1^2 x_4^2}{x_1^2 + x_2^2}} + x_4 V + x_1 v_1 + x_2 v_2 \leq 0 \right)$$

In[94]= Timing[Case16res = CylindricalDecomposition[

$$\begin{aligned} & \text{Ni} \ \&\& \ x1 > 0 \ \&\& \ x2 < 0 \ \&\& \ x4 \leq 0 \ \&\& \ \left( \forall_{\text{Eps}, \text{Eps} > 0} \exists_{\text{del}, \text{del} > 0} \text{Implies} \left[ \sqrt{x1^2 + x2^2 + 2 x4^2} < \text{del}, \right. \right. \\ & \quad -g1 x1 x4 - g2 x2 x4 + (x4 V + x1 v1 + x2 v2) \sqrt{x1^2 + x2^2} < \text{Eps} \sqrt{x1^2 + x2^2} \sqrt{x1^2 + x2^2 + 2 x4^2} \ \parallel \\ & \quad \left. \left. -g1 x1 x4 - g2 x2 x4 + (x4 V + x1 v1 + x2 v2) \sqrt{x1^2 + x2^2} \leq 0 \right] \right), \\ & \{x1, x2, x4, v1, v2, v3, V, g2, g1\}] \end{aligned}$$

Out[94]=

{207.875, x1 > 0 && x2 < 0 && x4 ≤ 0 && v1 == 0 && v2 == 0 && v3 ≤ 0 && ((V == 0 && g2 == 0 && g1 == 0) || (V > 0 && -V ≤ g2 ≤ V && -V ≤ g1 ≤ V))}

## Case 20:

In[95]= splt[GphCADSim[[20]]

Out[95]=

$$\begin{aligned} & \forall_{\text{Eps}, \text{Eps} > 0} \exists_{\text{del}, \text{del} > 0} \forall_{\{x1, x2, x4\}, x1 > 0 \ \&\& \ x2 > 0 \ \&\& \ x4 < 0 \ \&\& \ \sqrt{x1^2 + x2^2 + 2 x4^2} < \text{del}} \left( g1 \sqrt{\frac{x1^2 x4^2}{x1^2 + x2^2}} + \right. \\ & \quad g2 \sqrt{x4^2 - \frac{x1^2 x4^2}{x1^2 + x2^2}} + x4 V + x1 v1 + x2 v2 < \text{Eps} \sqrt{x1^2 + x2^2 + 2 x4^2} \ \parallel \\ & \quad \left. g1 \sqrt{\frac{x1^2 x4^2}{x1^2 + x2^2}} + g2 \sqrt{x4^2 - \frac{x1^2 x4^2}{x1^2 + x2^2}} + x4 V + x1 v1 + x2 v2 \leq 0 \right) \end{aligned}$$

In[96]= Timing[Case20res = CylindricalDecomposition[

$$\begin{aligned} & \text{Ni} \ \&\& \ x1 > 0 \ \&\& \ x2 > 0 \ \&\& \ x4 < 0 \ \&\& \ \left( \forall_{\text{Eps}, \text{Eps} > 0} \exists_{\text{del}, \text{del} > 0} \text{Implies} \left[ \sqrt{x1^2 + x2^2 + 2 x4^2} < \text{del}, \right. \right. \\ & \quad -g1 x1 x4 - g2 x2 x4 + (x4 V + x1 v1 + x2 v2) \sqrt{x1^2 + x2^2} < \text{Eps} \sqrt{x1^2 + x2^2} \sqrt{x1^2 + x2^2 + 2 x4^2} \ \parallel \\ & \quad \left. \left. -g1 x1 x4 - g2 x2 x4 + (x4 V + x1 v1 + x2 v2) \sqrt{x1^2 + x2^2} \leq 0 \right] \right), \\ & \{x1, x2, x4, v1, v2, v3, V, g2, g1\}] \end{aligned}$$

Out[96]=

{208.368, x1 > 0 && x2 > 0 && x4 < 0 && v1 == 0 && v2 == 0 && v3 ≤ 0 && ((V == 0 && g2 == 0 && g1 == 0) || (V > 0 && -V ≤ g2 ≤ V && -V ≤ g1 ≤ V))}

## List of the results

In[97]= Case1res

Out[97]=

x1 < 0 && x2 ≤ 0 && x4 ≤ 0 && v1 == 0 && v2 == 0 && v3 ≤ 0 && ((V == 0 && g2 == 0 && g1 == 0) || (V > 0 && -V ≤ g2 ≤ V && -V ≤ g1 ≤ V))

In[98]:= **Case3res**

Out[98]=

```
x1 < 0 && x2 > 0 && x4 < 0 && v1 == 0 && v2 == 0 && v3 ≤ 0 &&
((V == 0 && g2 == 0 && g1 == 0) || (V > 0 && -V ≤ g2 ≤ V && -V ≤ g1 ≤ V))
```

In[99]:= **Case16res**

Out[99]=

```
x1 > 0 && x2 < 0 && x4 ≤ 0 && v1 == 0 && v2 == 0 && v3 ≤ 0 &&
((V == 0 && g2 == 0 && g1 == 0) || (V > 0 && -V ≤ g2 ≤ V && -V ≤ g1 ≤ V))
```

In[100]:=

**Case20res**

Out[100]=

```
x1 > 0 && x2 > 0 && x4 < 0 && v1 == 0 && v2 == 0 && v3 ≤ 0 &&
((V == 0 && g2 == 0 && g1 == 0) || (V > 0 && -V ≤ g2 ≤ V && -V ≤ g1 ≤ V))
```

## Projections of x1, x2 and x4

In[101]:=

```
CylindricalDecomposition[Exists[{x1, x2, x4}, Case1res], {v1, v2, v3, V, g1, g2}]
(* Projection of these solutions on V,g1,g2 *)
```

Out[101]=

```
v1 == 0 && v2 == 0 && v3 ≤ 0 && ((V == 0 && g1 == 0 && g2 == 0) || (V > 0 && -V ≤ g1 ≤ V && -V ≤ g2 ≤ V))
```

In[102]:=

```
CylindricalDecomposition[Exists[{x1, x2, x4}, Case3res], {v1, v2, v3, V, g1, g2}]
```

Out[102]=

```
v1 == 0 && v2 == 0 && v3 ≤ 0 && ((V == 0 && g1 == 0 && g2 == 0) || (V > 0 && -V ≤ g1 ≤ V && -V ≤ g2 ≤ V))
```

In[103]:=

```
CylindricalDecomposition[Exists[{x1, x2, x4}, Case16res], {v1, v2, v3, V, g1, g2}]
```

Out[103]=

```
v1 == 0 && v2 == 0 && v3 ≤ 0 && ((V == 0 && g1 == 0 && g2 == 0) || (V > 0 && -V ≤ g1 ≤ V && -V ≤ g2 ≤ V))
```

In[104]:=

```
CylindricalDecomposition[Exists[{x1, x2, x4}, Case20res], {v1, v2, v3, V, g1, g2}]
```

Out[104]=

```
v1 == 0 && v2 == 0 && v3 ≤ 0 && ((V == 0 && g1 == 0 && g2 == 0) || (V > 0 && -V ≤ g1 ≤ V && -V ≤ g2 ≤ V))
```

(\*These conditions are all the same. They are already in N\_i. We can check it by adding these conditions to res and calculating N\_i again. \*)

## Update N\_i

In[105]:=

**Ni**

Out[105]=

```
v1 == 0 && v2 == 0 && v3 ≤ 0 && V ≥ 0 && -V ≤ g1 ≤ V && -V ≤ g2 ≤ V
```

In[106]:=

**AppendTo[res,**

$$v1 == 0 \ \&\& \ v2 == 0 \ \&\& \ v3 \leq 0 \ \&\& \ ((V == 0 \ \&\& \ g1 == 0 \ \&\& \ g2 == 0) \ || \ (V > 0 \ \&\& \ -V \leq g1 \leq V \ \&\& \ -V \leq g2 \leq V))$$

Out[106]=

$$\{v2 \leq 0 \ \&\& \ v1 \geq 0, \ v3 \leq 0 \ \&\& \ v2 \geq 0, \ g1 \geq -V, \ g1 \leq V, \ \text{True}, \ v3 \leq 0, \\ v2 \leq 0, \ v3 \leq 0 \ \&\& \ v2 \leq 0, \ g1 \leq V \ \&\& \ v1 \leq 0, \ v3 \leq 0 \ \&\& \ v1 \leq 0, \ v2 \leq 0 \ \&\& \ v1 \leq 0, \\ g2 \in \mathbb{R} \ \&\& \ V \geq -g2 \ \&\& \ v2 \geq 0, \ g2 \in \mathbb{R} \ \&\& \ V \geq g2 \ \&\& \ v2 \leq 0, \ v3 \leq 0, \ v3 \leq 0, \ v3 \leq 0, \ v3 \leq 0, \\ v1 == 0 \ \&\& \ v2 == 0 \ \&\& \ v3 \leq 0 \ \&\& \ ((V == 0 \ \&\& \ g1 == 0 \ \&\& \ g2 == 0) \ || \ (V > 0 \ \&\& \ -V \leq g1 \leq V \ \&\& \ -V \leq g2 \leq V))\}$$

In[107]:=

**CylindricalDecomposition[And @@ res, {v1, v2, v3, V, g1, g2}]**

Out[107]=

$$v1 == 0 \ \&\& \ v2 == 0 \ \&\& \ v3 \leq 0 \ \&\& \ ((V == 0 \ \&\& \ g1 == 0 \ \&\& \ g2 == 0) \ || \ (V > 0 \ \&\& \ -V \leq g1 \leq V \ \&\& \ -V \leq g2 \leq V))$$

## Last Unresolved Case : Case 9

In[108]:=

**GphCADSim[9]**

Out[108]=

$$x1 == 0 \ \&\& \ x2 == 0 \ \&\& \ x3 == 0 \ \&\& \ x4 < 0 \ \&\& \ x4 < x5 < -x4 \ \&\& \ -\sqrt{x4^2 - x5^2} \leq x6 \leq \sqrt{x4^2 - x5^2}$$

In[109]:=

**split[GphCADSim[9]]**

Out[109]=

$$\forall_{Eps, Eps > 0} \exists_{del, del > 0} \forall_{\{x4, x5, x6\}, x4 < 0 \ \&\& \ x4 < x5 < -x4 \ \&\& \ -\sqrt{x4^2 - x5^2} \leq x6 \leq \sqrt{x4^2 - x5^2} \ \&\& \ \sqrt{x4^2 + x5^2 + x6^2} < del \left( g1 x5 + \right. \\ \left. g2 x6 + x4 V < Eps \ \sqrt{x4^2 + x5^2 + x6^2} \ \ || \ g1 x5 + g2 x6 + x4 V \leq 0 \right)$$

(\* The condition  $x4 < 0 \ \&\& \ x4 < x5 < -x4 \ \&\&$

$-\sqrt{-x5^2 + x4^2} \leq x6 \leq \sqrt{-x5^2 + x4^2}$  is the same as  $x4 < 0$  and  $x6^2 + x5^2 \leq x4^2$  \*)

In[110]:=

$$\forall_{Eps, Eps > 0} \exists_{del, del > 0} \forall_{\{x4, x5, x6\}, x4 < 0 \ \&\& \ x6^2 + x5^2 \leq x4^2 \ \&\& \ \sqrt{x4^2 + x5^2 + x6^2} < del \left( g1 x5 + g2 x6 + x4 V < \right. \\ \left. Eps \ \sqrt{x4^2 + x5^2 + x6^2} \ \ || \ g1 x5 + g2 x6 + x4 V \leq 0 \right)$$

Out[110]=

$$\forall_{Eps, Eps > 0} \exists_{del, del > 0} \forall_{\{x4, x5, x6\}, x4 < 0 \ \&\& \ x5^2 + x6^2 \leq x4^2 \ \&\& \ \sqrt{x4^2 + x5^2 + x6^2} < del \left( g1 x5 + g2 x6 + x4 V < \right. \\ \left. Eps \ \sqrt{x4^2 + x5^2 + x6^2} \ \ || \ g1 x5 + g2 x6 + x4 V \leq 0 \right)$$

In[111]:=

**Reduce`ToPrenexForm[%]**

Out[111]=

$$\forall_{\{c_1\}} \exists_{\{c_2\}} \forall_{\{c_3, c_4, c_5\}} \left( (c_2 > 0 \ \&\& \ (c_3 \geq 0 \ \ || \ \sqrt{c_5^2 + c_3^2 + c_4^2} \geq c_2 \ \ || \right. \\ \left. g2 c_5 + g1 c_4 + c_3 V < c_1 \ \sqrt{c_5^2 + c_3^2 + c_4^2} \ \ || \ c_5^2 + c_4^2 > c_3^2 \ \ || \ g2 c_5 + g1 c_4 + c_3 V \leq 0) \right) \ \ || \ c_1 \leq 0$$

In[112]:=

$$\forall_{\{c_1\}} \exists_{\{c_2\}} \forall_{\{c_3, c_4, c_5\}} \left( (c_2 > 0 \ \&\& \ (c_3 \geq 0 \ \parallel \ \sqrt{c_5^2 + c_3^2 + c_4^2} \geq c_2 \ \parallel \right. \\ \left. g_2 c_5 + g_1 c_4 + c_3 V < c_1 \ \sqrt{c_5^2 + c_3^2 + c_4^2} \ \parallel \ c_5^2 + c_4^2 > c_3^2 \ \parallel \ g_2 c_5 + g_1 c_4 + c_3 V \leq 0) \right) \parallel c_1 \leq 0 \Big) /. \\ \{C[1] \rightarrow \text{Eps}, C[2] \rightarrow \text{del}, C[3] \rightarrow x_4, C[4] \rightarrow x_5, C[5] \rightarrow x_6\}$$

Out[112]=

$$\forall_{\{\text{Eps}\}} \exists_{\{\text{del}\}} \forall_{\{x_4, x_5, x_6\}} \left( (\text{del} > 0 \ \&\& \ (x_4 \geq 0 \ \parallel \ \sqrt{x_4^2 + x_5^2 + x_6^2} \geq \text{del} \ \parallel \right. \\ \left. g_1 x_5 + g_2 x_6 + x_4 V < \text{Eps} \ \sqrt{x_4^2 + x_5^2 + x_6^2} \ \parallel \ x_5^2 + x_6^2 > x_4^2 \ \parallel \ g_1 x_5 + g_2 x_6 + x_4 V \leq 0) \right) \parallel \text{Eps} \leq 0 \Big)$$

(\* Finding a point that suggests that the this cell might refine the upper estimate to the normal cone: Ni\*)

In[113]:=

Ni

Out[113]=

$$v_1 == 0 \ \&\& \ v_2 == 0 \ \&\& \ v_3 \leq 0 \ \&\& \ V \geq 0 \ \&\& \ -V \leq g_1 \leq V \ \&\& \ -V \leq g_2 \leq V$$

In[114]:=

FindInstance[

$$\text{Eps} > 0 \ \&\& \ \text{del} > 0 \ \&\& \ \text{Not} \left[ (x_4 \geq 0 \ \parallel \ \sqrt{x_4^2 + x_5^2 + x_6^2} \geq \text{del} \ \parallel \ g_1 x_5 + g_2 x_6 + x_4 V < \text{Eps} \ \sqrt{x_4^2 + x_5^2 + x_6^2} \ \parallel \right. \\ \left. x_5^2 + x_6^2 > x_4^2 \ \parallel \ g_1 x_5 + g_2 x_6 + x_4 V \leq 0) \right] \ \&\& \ \text{Ni}, \\ \{v_1, v_2, v_3, V, g_1, g_2, \text{Eps}, \text{del}, x_1, x_2, x_3, x_4, x_5, x_6\}, \text{Reals}]$$

Out[114]=

$$\left\{ \left\{ v_1 \rightarrow 0, v_2 \rightarrow 0, v_3 \rightarrow -1, V \rightarrow 1, g_1 \rightarrow -\frac{13}{16}, g_2 \rightarrow -\frac{15}{16}, \text{Eps} \rightarrow \frac{5}{256}, \right. \right. \\ \left. \left. \text{del} \rightarrow 2, x_1 \rightarrow \frac{171}{10}, x_2 \rightarrow -\frac{103}{5}, x_3 \rightarrow -\frac{15}{2}, x_4 \rightarrow -1, x_5 \rightarrow -\frac{1}{2}, x_6 \rightarrow -\frac{11}{16} \right\} \right\}$$

(\* Now we know that this cell might refine the upper estimate Ni, we start dissecting this cell and do QE on pieces of it. \*)

Focus on the Boundary of Case 9 First: when  $x_6^2 + x_5^2 == x_4^2$

**Key take away** is that lower number of variables to eliminate is better chances for QE termination.

(\* Positive x6 Root\*)

In[115]:=

$$\forall_{\{\text{Eps}, \text{Eps} > 0\}} \exists_{\{\text{del}, \text{del} > 0\}} \forall_{\{x_5, x_4\}, x_4 < 0 \ \&\& \ x_4 < x_5 < -x_4 \ \&\& \ \sqrt{x_5^2 + x_6^2 + x_4^2} < \text{del}} \left( x_4 V + x_5 g_1 + x_6 g_2 < \text{Eps} \ \sqrt{x_5^2 + x_6^2 + x_4^2} \ \parallel \right. \\ \left. x_4 V + x_5 g_1 + x_6 g_2 \leq 0 \right) /. \ x_6 \rightarrow \sqrt{-x_5^2 + x_4^2} \ /. \ \sqrt{x_4^2} \rightarrow -x_4$$

Out[115]=

$$\forall_{\{\text{Eps}, \text{Eps} > 0\}} \exists_{\{\text{del}, \text{del} > 0\}} \forall_{\{x_5, x_4\}, x_4 < 0 \ \&\& \ x_4 < x_5 < -x_4 \ \&\& \ -\sqrt{2} \ x_4 < \text{del}} \left( g_1 x_5 + g_2 \sqrt{-x_5^2 + x_4^2} + x_4 V < -\sqrt{2} \ \text{Eps} \ x_4 \ \parallel \right. \\ \left. g_1 x_5 + g_2 \sqrt{-x_5^2 + x_4^2} + x_4 V \leq 0 \right)$$

In[116]:=

**Timing[Resolve[%, Reals]]**

Out[116]=

$$\{32.2965, (g2 \leq 0 \ \&\& \ ((g1 \leq 0 \ \&\& \ V \geq -g1) \parallel (g1 > 0 \ \&\& \ V \geq g1)) \parallel (g2 > 0 \ \&\& \ V \geq \sqrt{g1^2 + g2^2}))\}$$

In[117]:=

**CylindricalDecomposition[**

$$(g2 \leq 0 \ \&\& \ ((g1 \leq 0 \ \&\& \ V \geq -g1) \parallel (g1 > 0 \ \&\& \ V \geq g1)) \parallel (g2 > 0 \ \&\& \ V \geq \sqrt{g1^2 + g2^2}), \{V, g1, g2\}]$$

Out[117]=

$$(V == 0 \ \&\& \ g1 == 0 \ \&\& \ g2 \leq 0) \parallel$$

$$(V > 0 \ \&\& \ ((g1 == -V \ \&\& \ g2 \leq 0) \parallel (-V < g1 < V \ \&\& \ g2 \leq \sqrt{-g1^2 + V^2}) \parallel (g1 == V \ \&\& \ g2 \leq 0)))$$

**(\*Negative x6 Root:\*)**

In[118]:=

$$\forall_{Eps, Eps > 0} \exists_{del, del > 0} \forall_{\{x5, x4\}, x4 < 0 \ \&\& \ x4 < x5 < -x4 \ \&\& \ \sqrt{x5^2 + x6^2 + x4^2} < del} (x4 V + x5 g1 + x6 g2 < Eps \ \sqrt{x5^2 + x6^2 + x4^2} \parallel x4 V + x5 g1 + x6 g2 \leq 0) / . \ x6 \rightarrow -\sqrt{-x5^2 + x4^2} / . \ \sqrt{x4^2} \rightarrow -x4$$

Out[118]=

$$\forall_{Eps, Eps > 0} \exists_{del, del > 0} \forall_{\{x5, x4\}, x4 < 0 \ \&\& \ x4 < x5 < -x4 \ \&\& \ -\sqrt{2} \ x4 < del} (g1 x5 - g2 \sqrt{-x5^2 + x4^2} + x4 V < -\sqrt{2} \ Eps \ x4 \parallel g1 x5 - g2 \sqrt{-x5^2 + x4^2} + x4 V \leq 0)$$

In[119]:=

**Timing[Resolve[%, Reals]]**

Out[119]=

$$\{26.7179, (g2 < 0 \ \&\& \ V \geq \sqrt{g1^2 + g2^2}) \parallel (g2 == 0 \ \&\& \ ((g1 < 0 \ \&\& \ V \geq \sqrt{g1^2}) \parallel (g1 == 0 \ \&\& \ V \geq 0) \parallel (g1 > 0 \ \&\& \ V \geq \sqrt{g1^2}))) \parallel (g2 > 0 \ \&\& \ ((g1 \leq 0 \ \&\& \ V \geq -g1) \parallel (g1 > 0 \ \&\& \ V \geq g1)))\}$$

In[120]:=

**CylindricalDecomposition[**

$$(g2 < 0 \ \&\& \ V \geq \sqrt{g1^2 + g2^2}) \parallel (g2 == 0 \ \&\& \ ((g1 < 0 \ \&\& \ V \geq \sqrt{g1^2}) \parallel (g1 == 0 \ \&\& \ V \geq 0) \parallel (g1 > 0 \ \&\& \ V \geq \sqrt{g1^2}))) \parallel (g2 > 0 \ \&\& \ ((g1 \leq 0 \ \&\& \ V \geq -g1) \parallel (g1 > 0 \ \&\& \ V \geq g1)), \{V, g1, g2\}]$$

Out[120]=

$$(V == 0 \ \&\& \ g1 == 0 \ \&\& \ g2 \geq 0) \parallel$$

$$(V > 0 \ \&\& \ ((g1 == -V \ \&\& \ g2 \geq 0) \parallel (-V < g1 < V \ \&\& \ g2 \geq -\sqrt{-g1^2 + V^2}) \parallel (g1 == V \ \&\& \ g2 \geq 0)))$$

## Update N<sub>i</sub>

In[121]:=

```
AppendTo[res, (g2 ≤ 0 && ((g1 ≤ 0 && V ≥ -g1) || (g1 > 0 && V ≥ g1))) || (g2 > 0 && V ≥ √(g12 + g22))];
AppendTo[res, (g2 < 0 && V ≥ √(g12 + g22)) ||
  (g2 == 0 && ((g1 < 0 && V ≥ √(g12)) || (g1 == 0 && V ≥ 0) || (g1 > 0 && V ≥ √(g12)))) ||
  (g2 > 0 && ((g1 ≤ 0 && V ≥ -g1) || (g1 > 0 && V ≥ g1))];
```

In[123]:=

**res**

Out[123]=

```
{v2 ≤ 0 && v1 ≥ 0, v3 ≤ 0 && v2 ≥ 0, g1 ≥ -V, g1 ≤ V, True, v3 ≤ 0,
  v2 ≤ 0, v3 ≤ 0 && v2 ≤ 0, g1 ≤ V && v1 ≤ 0, v3 ≤ 0 && v1 ≤ 0, v2 ≤ 0 && v1 ≤ 0,
  g2 ∈ ℝ && V ≥ -g2 && v2 ≥ 0, g2 ∈ ℝ && V ≥ g2 && v2 ≤ 0, v3 ≤ 0, v3 ≤ 0, v3 ≤ 0, v3 ≤ 0,
  v1 == 0 && v2 == 0 && v3 ≤ 0 && (V == 0 && g1 == 0 && g2 == 0) || (V > 0 && -V ≤ g1 ≤ V && -V ≤ g2 ≤ V),
  (g2 ≤ 0 && ((g1 ≤ 0 && V ≥ -g1) || (g1 > 0 && V ≥ g1))) || (g2 > 0 && V ≥ √(g12 + g22)),
  (g2 < 0 && V ≥ √(g12 + g22)) || (g2 == 0 && ((g1 < 0 && V ≥ √(g12)) || (g1 == 0 && V ≥ 0) || (g1 > 0 && V ≥ √(g12)))) ||
  (g2 > 0 && ((g1 ≤ 0 && V ≥ -g1) || (g1 > 0 && V ≥ g1))}
```

In[124]:=

**Reduce[And@@res, Reals]**

Out[124]=

```
((g2 < 0 && V ≥ √(g12 + g22) && v3 ≤ 0) || (g2 == 0 &&
  ((g1 < 0 && V ≥ √(g12) && v3 ≤ 0) || (g1 == 0 && V ≥ 0 && v3 ≤ 0) || (g1 > 0 && V ≥ √(g12) && v3 ≤ 0))) ||
  (g2 > 0 && V ≥ √(g12 + g22) && v3 ≤ 0) && v2 == 0 && v1 == 0
```

(\* Check that the new Normal cone upper estimate found by Reduce[And@@res,Reals] above is sharper than the previous upper estimate by finding a point inside the old upper bound and outside of the new one: \*)

In[125]:=

**FindInstance[Not[%]&&Ni, {v1, v2, v3, V, g1, g2}]**

Out[125]=

```
{{v1 → 0, v2 → 0, v3 → -1, V → 17/8, g1 → -1, g2 → -2}}
```

(\* Hence we update the upper estimate to the new set of conditions. This is (5.5) on the paper.\*)

In[126]:=

Ni = Reduce[And @@ res, Reals]

Out[126]=

$$\left( (g_2 < 0 \ \&\& \ V \geq \sqrt{g_1^2 + g_2^2} \ \&\& \ v_3 \leq 0) \parallel (g_2 == 0 \ \&\& \ \left( (g_1 < 0 \ \&\& \ V \geq \sqrt{g_1^2} \ \&\& \ v_3 \leq 0) \parallel (g_1 == 0 \ \&\& \ V \geq 0 \ \&\& \ v_3 \leq 0) \parallel (g_1 > 0 \ \&\& \ V \geq \sqrt{g_1^2} \ \&\& \ v_3 \leq 0) \right) \parallel (g_2 > 0 \ \&\& \ V \geq \sqrt{g_1^2 + g_2^2} \ \&\& \ v_3 \leq 0) \right) \ \&\& \ v_2 == 0 \ \&\& \ v_1 == 0$$

In[127]:=

CylindricalDecomposition[Ni, {v1, v2, v3, V, g1, g2}]

Out[127]=

$$v_1 == 0 \ \&\& \ v_2 == 0 \ \&\& \ v_3 \leq 0 \ \&\& \ \left( (V == 0 \ \&\& \ g_1 == 0 \ \&\& \ g_2 == 0) \parallel (V > 0 \ \&\& \ \left( (g_1 == -V \ \&\& \ g_2 == 0) \parallel (-V < g_1 < V \ \&\& \ -\sqrt{-g_1^2 + V^2} \leq g_2 \leq \sqrt{-g_1^2 + V^2}) \parallel (g_1 == V \ \&\& \ g_2 == 0) \right) \right)$$

## Last Case checked against Ni

(\*)

Check if the conditions of this cell possibly refines the upper estimate of the normal cone  $N_i$  in any way. We check, if there can be possibly be any point in the current  $N_i$  that doesn't satisfy the conditions cell9 imposes, but looking for any point in " $N_i \ \&\& \ \text{Not}[\text{NormalToCell9}]$ ".

\*)

In[128]:=

NotNormalToCell9 = Reduce`ToPrenexForm[Not[splt[GphCADSim[9]]]]

Out[128]=

$$\exists_{\{c_1\}} \forall_{\{c_2\}} \exists_{\{c_3, c_4, c_5\}} \left( c_1 > 0 \ \&\& \ \left( (c_3 < 0 \ \&\& \ c_3 < c_4 \ \&\& \ c_4 < -c_3 \ \&\& \ \sqrt{c_5^2 + c_3^2 + c_4^2} < c_2 \ \&\& \ g_2 c_5 + g_1 c_4 + c_3 V \geq c_1 \sqrt{c_5^2 + c_3^2 + c_4^2} \ \&\& \ -\sqrt{c_3^2 - c_4^2} \leq c_5 \ \&\& \ c_5 \leq \sqrt{c_3^2 - c_4^2} \ \&\& \ g_2 c_5 + g_1 c_4 + c_3 V > 0) \parallel c_2 \leq 0 \right) \right)$$

In[129]:=

NotNormalToCell9InnerFormulaQuantFree =

$$\left( c_1 > 0 \ \&\& \ \left( (c_3 < -c_5 \ \&\& \ c_5 < 0 \ \&\& \ c_5 < c_3 \ \&\& \ \sqrt{c_5^2 + c_3^2 + c_4^2} < c_2 \ \&\& \ c_5 V + c_3 g_1 + c_4 g_2 \geq c_1 \sqrt{c_5^2 + c_3^2 + c_4^2} \ \&\& \ c_4 \leq \sqrt{c_5^2 - c_3^2} \ \&\& \ -\sqrt{c_5^2 - c_3^2} \leq c_4 \ \&\& \ c_5 V + c_3 g_1 + c_4 g_2 > 0) \parallel c_2 \leq 0 \right) \right)$$

Out[129]=

$$c_1 > 0 \ \&\& \ \left( (c_3 < -c_5 \ \&\& \ c_5 < 0 \ \&\& \ c_5 < c_3 \ \&\& \ \sqrt{c_3^2 + c_4^2 + c_5^2} < c_2 \ \&\& \ g_1 c_3 + g_2 c_4 + V c_5 \geq c_1 \sqrt{c_3^2 + c_4^2 + c_5^2} \ \&\& \ c_4 \leq \sqrt{-c_3^2 + c_5^2} \ \&\& \ -\sqrt{-c_3^2 + c_5^2} \leq c_4 \ \&\& \ g_1 c_3 + g_2 c_4 + V c_5 > 0) \parallel c_2 \leq 0 \right)$$

(\*) The relevant clause for  $\text{Epsilon} (=C[1]) > 0$  and  $\text{Delta} (=C[2]) > 0$  \*)

In[130]:=

```
NotNormalToCell9InnerFormulaQuantFreeNonNegEpsNonNegDel =
  (c3 < -c5 && c5 < 0 && c5 < c3 && sqrt(c5^2 + c3^2 + c4^2) < c2 && c5 V + c3 g1 + c4 g2 >= c1 sqrt(c5^2 + c3^2 + c4^2) &&
  c4 <= sqrt(c5^2 - c3^2) && -sqrt(c5^2 - c3^2) <= c4 && c5 V + c3 g1 + c4 g2 > 0) && C[1] >= 0 && C[2] > 0
```

Out[130]=

```
c3 < -c5 && c5 < 0 && c5 < c3 && sqrt(c3^2 + c4^2 + c5^2) < c2 && g1 c3 + g2 c4 + V c5 >= c1 sqrt(c3^2 + c4^2 + c5^2) &&
  c4 <= sqrt(-c3^2 + c5^2) && -sqrt(-c3^2 + c5^2) <= c4 && g1 c3 + g2 c4 + V c5 > 0 && c1 >= 0 && c2 > 0
```

(\* Upper estimate N\_i: \*)

In[131]:=

Ni

Out[131]=

```
((g2 < 0 && V >= sqrt(g1^2 + g2^2) && v3 <= 0) || (g2 == 0 &&
  ((g1 < 0 && V >= sqrt(g1^2) && v3 <= 0) || (g1 == 0 && V >= 0 && v3 <= 0) || (g1 > 0 && V >= sqrt(g1^2) && v3 <= 0))) ||
  (g2 > 0 && V >= sqrt(g1^2 + g2^2) && v3 <= 0)) && v2 == 0 && v1 == 0
```

(\* There are no points that are in Ni but that does not satisfy this clause: \*)

In[133]:=

```
Timing[FindInstance[Ni && NotNormalToCell9InnerFormulaQuantFreeNonNegEpsNonNegDel,
  {v1, v2, v3, V, g1, g2, C[1], C[2], C[3], C[4], C[5], C[6]}, Reals]]
```

Out[133]=

```
{7.38176, {}}
```

(\* No point can be found, indicating this formula Unsatisfiable.

Hence, no condition that Cell9 imposes shrink the size of N\_i.

Hence, now that all the cases are solved,  
we have gone through all the cells in the CAD of C,  
and we now have N\_i = N\_c.

\*)

# Section 7 : Showing $P = C$

## P and its projection:

In[134]:=

```

P = And@@ { (v1^2 + v2^2 + v3^2) + (g1^2 + g2^2 + V^2) ≤ 1 , (p1^2 + p2^2) ≤ 1 ,
  (v1^2 + v2^2) p1^2 == v1^2 , (v1^2 + v2^2) p2^2 == v2^2 ,
  v1 p1 ≥ 0 ,
  v2 p2 ≥ 0 ,
  g1 == -V p1 ,
  g2 == -V p2 ,
  v3 ≥ 0 ,
  V ≤ 0 ,
  v3 V == 0 }

```

Out[134]=

```

g1^2 + g2^2 + V^2 + v1^2 + v2^2 + v3^2 ≤ 1 && p1^2 + p2^2 ≤ 1 && p1^2 (v1^2 + v2^2) == v1^2 && p2^2 (v1^2 + v2^2) == v2^2 &&
p1 v1 ≥ 0 && p2 v2 ≥ 0 && g1 == -p1 V && g2 == -p2 V && v3 ≥ 0 && V ≤ 0 && V v3 == 0

```

In[135]:=

```

Timing[rel = Resolve[Exists[{p1, p2}, P]]] (* Proj of P on p1, p2 *)

```

Out[135]=

```

{0.161748, (g1 | g2 | v1 | v2) ∈ ℝ &&
  ((g1 == 0 && g2 == 0 && V == 0 && v1 == 0 && v2 ≥ 0 && v3 ≥ 0 && g1^2 + g2^2 + V^2 + v1^2 + v2^2 + v3^2 ≤ 1) ||
  (g1 == 0 && g2 == 0 && V == 0 && v1 == 0 && v2 ≤ 0 && v3 ≥ 0 && g1^2 + g2^2 + V^2 + v1^2 + v2^2 + v3^2 ≤ 1) ||
  (g1 == 0 && g2 == 0 && V == 0 && v1 == 0 && v2 == 0 && v3 ≥ 0 && g1^2 + g2^2 + V^2 + v1^2 + v2^2 + v3^2 ≤ 1) ||
  (V < 0 && g1^2 + g2^2 - V^2 ≤ 0 && g1 v1 ≥ 0 && g2 v2 ≥ 0 && g1^2 v1^2 - V^2 v1^2 + g1^2 v2^2 == 0 &&
  g2^2 v1^2 + g2^2 v2^2 - V^2 v2^2 == 0 && v3 == 0 && g1^2 + g2^2 + V^2 + v1^2 + v2^2 + v3^2 ≤ 1) ||
  (g1 == 0 && g2 == 0 && V == 0 && v1 ≥ 0 && v2 == 0 && v1^2 + v2^2 > 0 && v3 ≥ 0 &&
  g1^2 + g2^2 + V^2 + v1^2 + v2^2 + v3^2 ≤ 1) || (g1 == 0 && g2 == 0 && V == 0 && v1 ≤ 0 &&
  v2 == 0 && v1^2 + v2^2 > 0 && v3 ≥ 0 && g1^2 + g2^2 + V^2 + v1^2 + v2^2 + v3^2 ≤ 1) ||
  (g1 == 0 && g2 == 0 && V == 0 && v1 ≥ 0 && v2 ≥ 0 && v1^2 + v2^2 > 0 && v3 ≥ 0 &&
  g1^2 + g2^2 + V^2 + v1^2 + v2^2 + v3^2 ≤ 1) || (g1 == 0 && g2 == 0 && V == 0 && v1 == 0 &&
  v2 ≥ 0 && v1^2 + v2^2 > 0 && v3 ≥ 0 && g1^2 + g2^2 + V^2 + v1^2 + v2^2 + v3^2 ≤ 1) ||
  (g1 == 0 && g2 == 0 && V == 0 && v1 ≤ 0 && v2 ≥ 0 && v1^2 + v2^2 > 0 && v3 ≥ 0 &&
  g1^2 + g2^2 + V^2 + v1^2 + v2^2 + v3^2 ≤ 1) || (g1 == 0 && g2 == 0 && V == 0 && v1 ≥ 0 &&
  v2 ≤ 0 && v1^2 + v2^2 > 0 && v3 ≥ 0 && g1^2 + g2^2 + V^2 + v1^2 + v2^2 + v3^2 ≤ 1) ||
  (g1 == 0 && g2 == 0 && V == 0 && v1 ≥ 0 && v2 == 0 && v1^2 + v2^2 > 0 && v3 ≥ 0 &&
  g1^2 + g2^2 + V^2 + v1^2 + v2^2 + v3^2 ≤ 1) || (g1 == 0 && g2 == 0 && V == 0 && v1 == 0 &&
  v2 ≤ 0 && v1^2 + v2^2 > 0 && v3 ≥ 0 && g1^2 + g2^2 + V^2 + v1^2 + v2^2 + v3^2 ≤ 1) ||
  (g1 == 0 && g2 == 0 && V == 0 && v1 ≤ 0 && v2 ≤ 0 && v1^2 + v2^2 > 0 && v3 ≥ 0 &&

```



## C intersected with $B_1(0)$ (which we call re2 here)

In[140]:=

```
re2 = Simplify[(
  V ≤ 0 &&
  v3 ≥ 0 &&
  ((v1^2 + v2^2 == 0 && g1^2 + g2^2 ≤ V^2) ||
   (v1^2 + v2^2 ≠ 0 && g1 == -V v1 / Sqrt[(v1^2 + v2^2)] && g2 == -V v2 / Sqrt[(v1^2 + v2^2)]))
  && ((v3 == 0 && V ≤ 0) || (v3 > 0 && V == 0))
) (* <- gph(Q) *)
&&
g1^2 + g2^2 + V^2 + v1^2 + v2^2 + v3^2 ≤ 1 (*<- B_1(0)*)
]
```

Out[140]=

$$V \leq 0 \ \&\& \ v3 \geq 0 \ \&\& \ g1^2 + g2^2 + V^2 + v1^2 + v2^2 + v3^2 \leq 1 \ \&\& \\ \left( (g1^2 + g2^2 \leq V^2 \ \&\& \ v1^2 + v2^2 == 0) \ \parallel \left( v1^2 + v2^2 \neq 0 \ \&\& \ g1 + \frac{V v1}{\sqrt{v1^2 + v2^2}} == 0 \ \&\& \ g2 + \frac{V v2}{\sqrt{v1^2 + v2^2}} == 0 \right) \right) \ \&\& \\ (V \geq 0 \ \parallel \ v3 \leq 0)$$

## Proving that they are the same

In[141]:=

```
Timing[Reduce[re1 && Not[re2]]] (* There is no point in proj(P) that is not in gph(Q) ∩ B_1(0) *)
```

Out[141]=

```
{2.04372, False}
```

In[142]:=

```
Timing[Reduce[Simplify[Not[re1] && re2]]]
(* There is no point in gph(Q) ∩ B_1(0) that is not in proj(P) *)
```

Out[142]=

```
{0.995868, False}
```
